# Supplementary material for: Variational Autoencoder Framework for Hyperspectral Retrievals (Hyper-VAE) of Phytoplankton Absorption and Chlorophyll a in Coastal Waters for NASA's EMIT and PACE Missions
Source: arXiv:2504.13476 source file (2025-04-18)
Supplement: Supplementary file 1 [file Appendix.tex]

\section*{Appendix}
\label{sec:appendix}

\subsection{Evaluations of $\mathit{a}_{ph}$ Predictions}
\label{app:1}

Moreover, this study aims to develop advanced algorithms for NASA’s current hyperspectral missions, including PACE and EMIT. 
After initial testing on HICO, we further evaluate our VAE-$a_{phy}$ using PACE and EMIT wavelengths with longer and shorter vector inputs to the VAE model, respectively. 
Figure~\ref{fig:PACE_EMIT_plots} exhibits the performance of our VAE-$a_{phy}$ and MDN models.
We can observe that our VAE-$a_{phy}$ consistently outperforms the MDN model across all metrics for both PACE and EMIT wavelength standards.
Regarding the prediction errors, the VAE always yields an MAE less than 1.30 while the MDN results in an MAE larger than 1.40, indicating that our VAE-$a_{phy}$ can provide more precise predictions on all PACE and EMIT wavelength standards.
The other two prediction error metrics, RMSE and RMSLE, show similar better performance.
Considering the prediction deviation, our VAE-$a_{phy}$ can still achieve a better bias and slope value (i.e., closer to zero) than the MDN.
These consistently superior performances on different metrics comprehensively highlight the advanced prediction capability of our VAE-$a_{phy}$ on the current new hyperspectral space mission, PACE and EMIT, demonstrating its robust generalization ability.

\begin{figure*}[h]
	\centering
	\subfigure[VAE on PACE 440nm]{
		\includegraphics[width=0.22\linewidth]{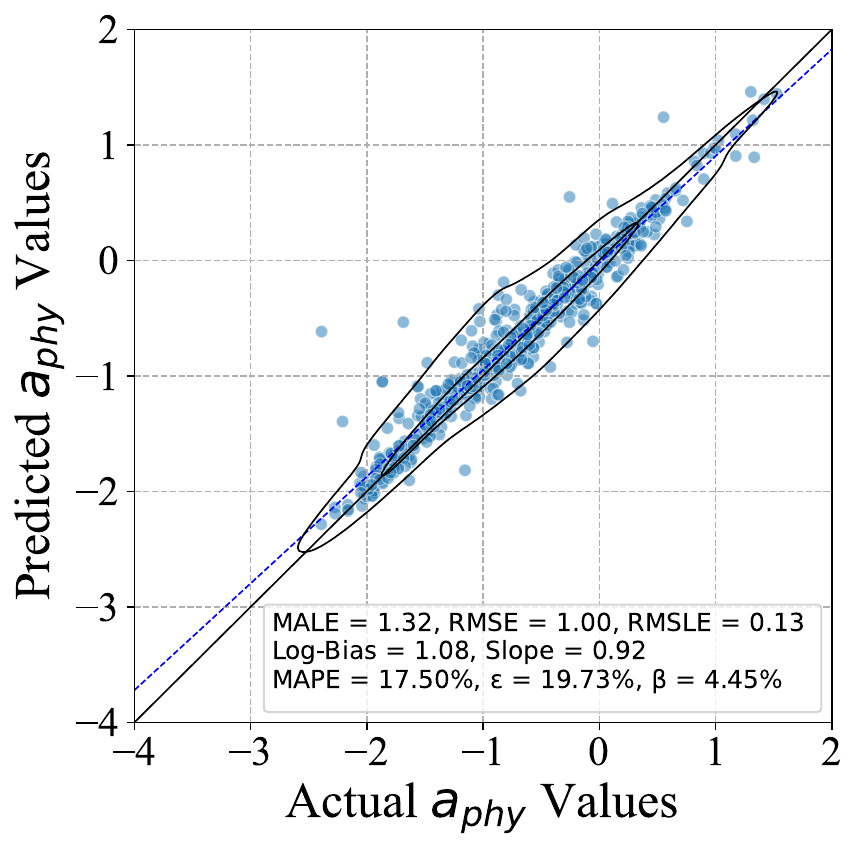}
		\label{Fig:PACE_3_plots1}
	}	
        \subfigure[MDN on PACE 440nm]{
		\includegraphics[width=0.22\linewidth]{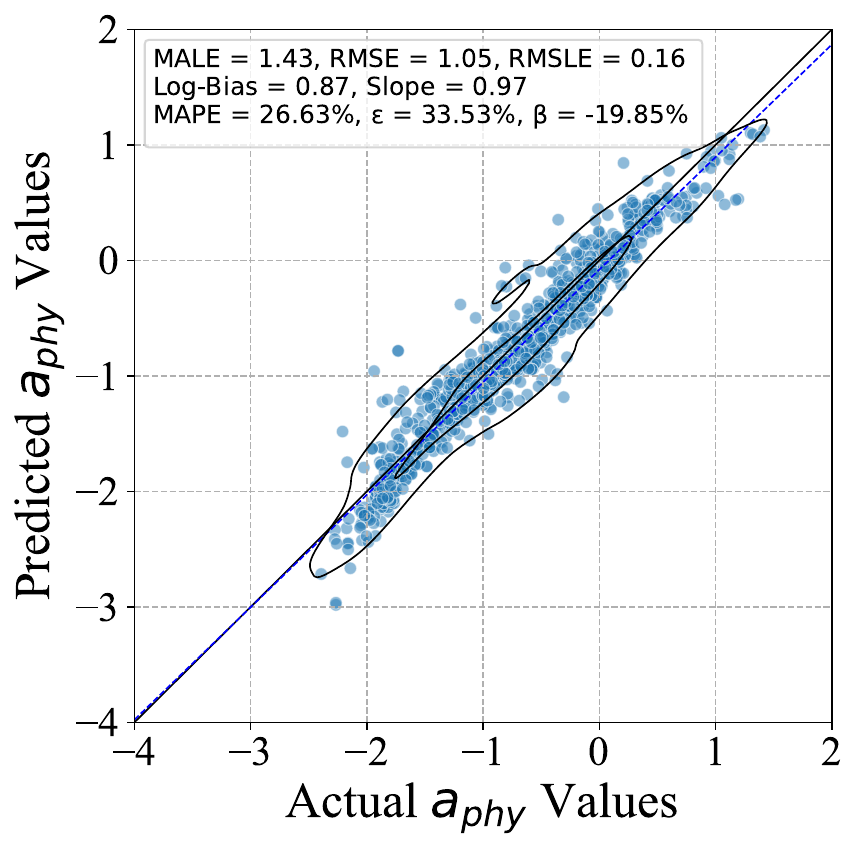}
		\label{Fig:PACE_3_plots4}
	}
 	\subfigure[VAE on EMIT 440nm]{
		\includegraphics[width=0.22\linewidth]{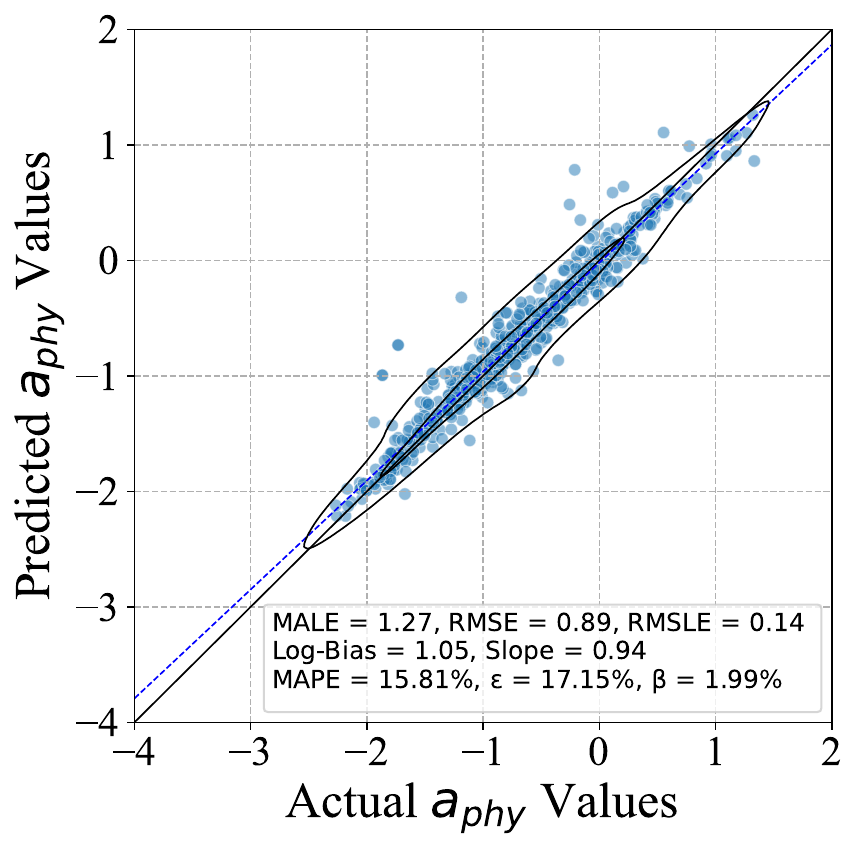}
		\label{Fig:EMIT_3_plots1}
	}	
 	\subfigure[MDN on EMIT 440nm]{
		\includegraphics[width=0.22\linewidth]{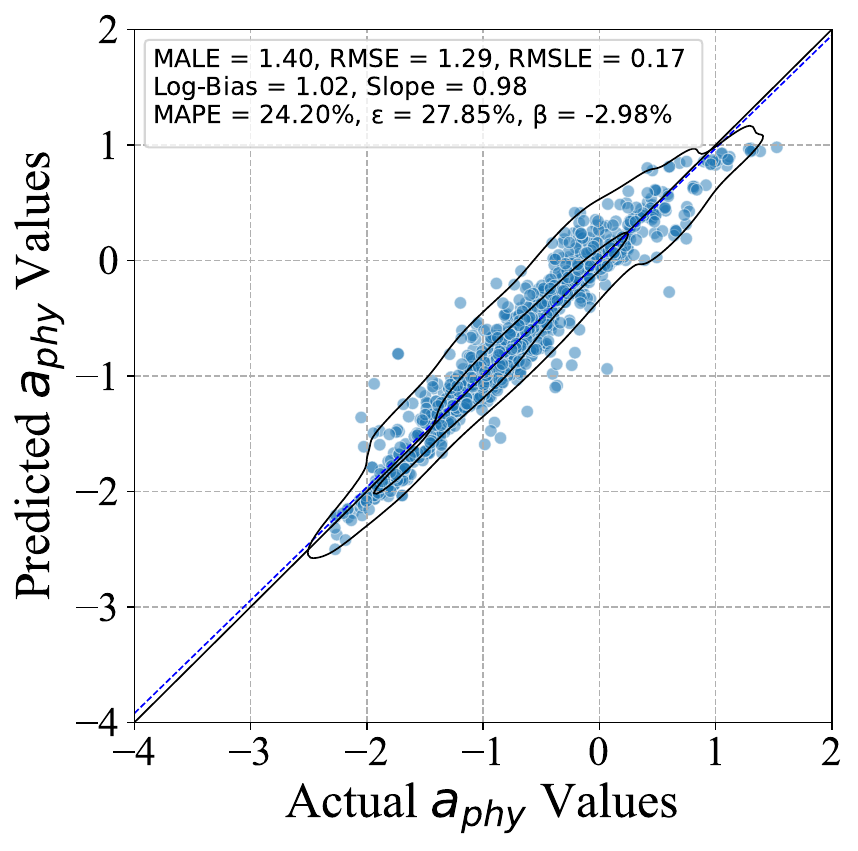}
		\label{Fig:EMIT_3_plots4}
	}
	\subfigure[VAE on PACE 620nm]{
		\includegraphics[width=0.22\linewidth]{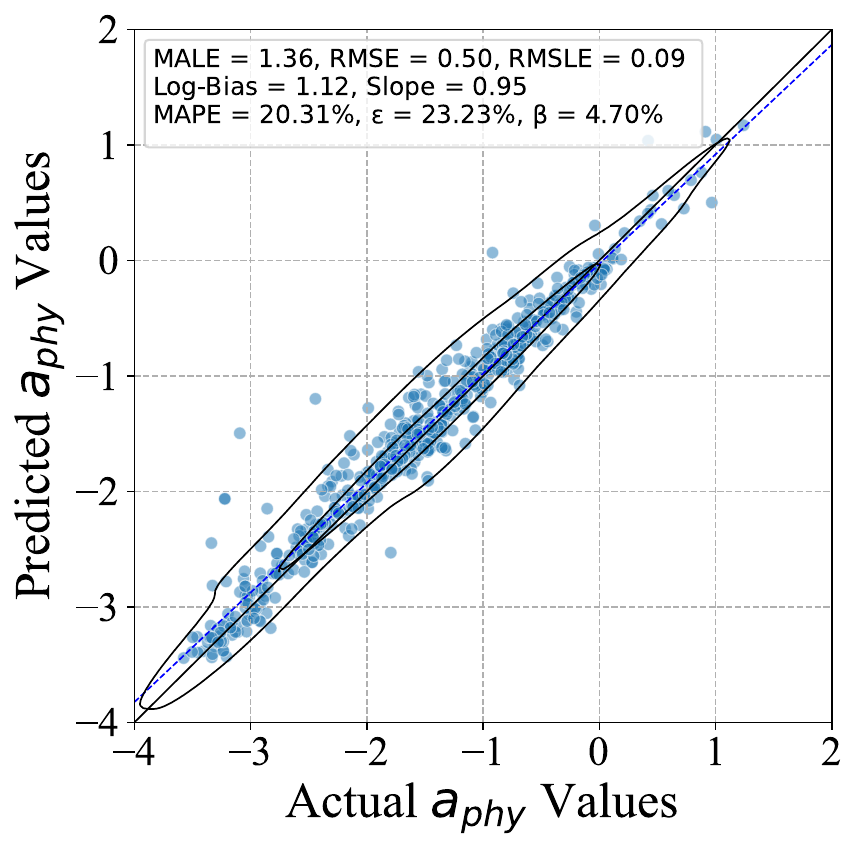}
		\label{Fig:PACE_3_plots2}
	}
 	\subfigure[MDN on PACE 620nm]{
		\includegraphics[width=0.22\linewidth]{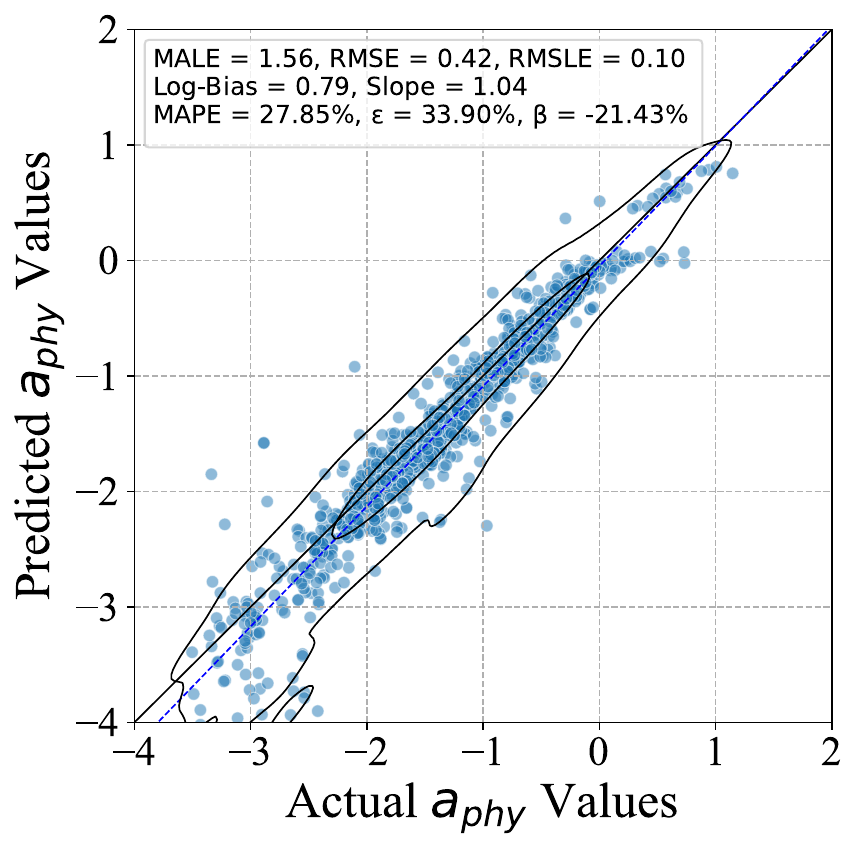}
		\label{Fig:PACE_3_plots5}
	}	
 	\subfigure[VAE on EMIT 618nm]{
		\includegraphics[width=0.22\linewidth]{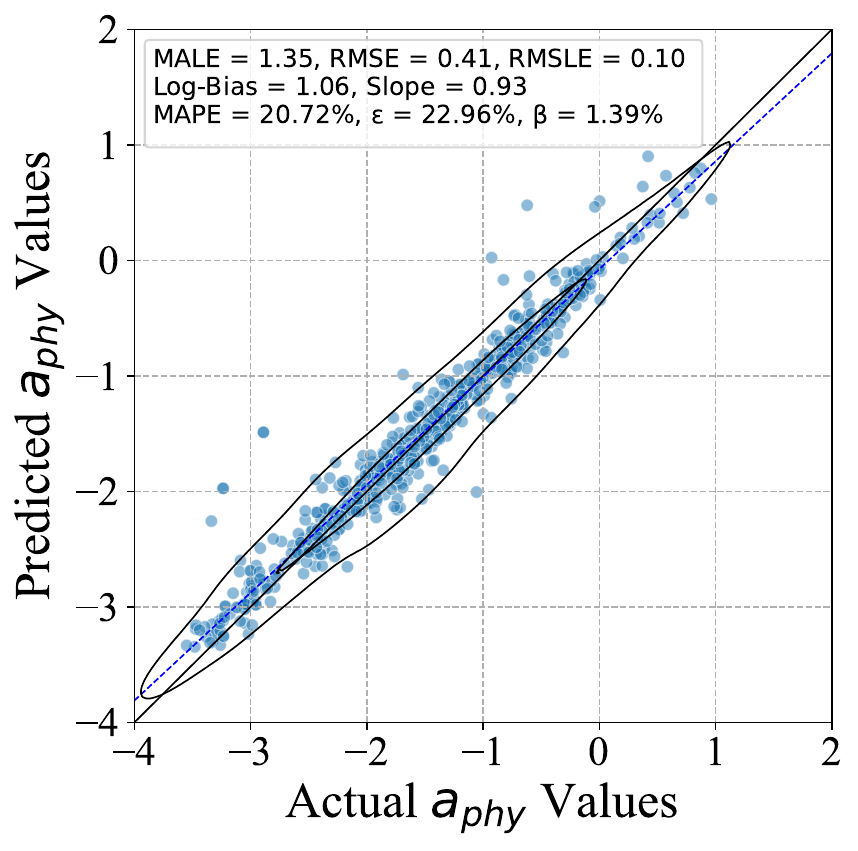}
		\label{Fig:EMIT_3_plots2}
	}
	\subfigure[MDN on EMIT 618nm]{
		\includegraphics[width=0.22\linewidth]{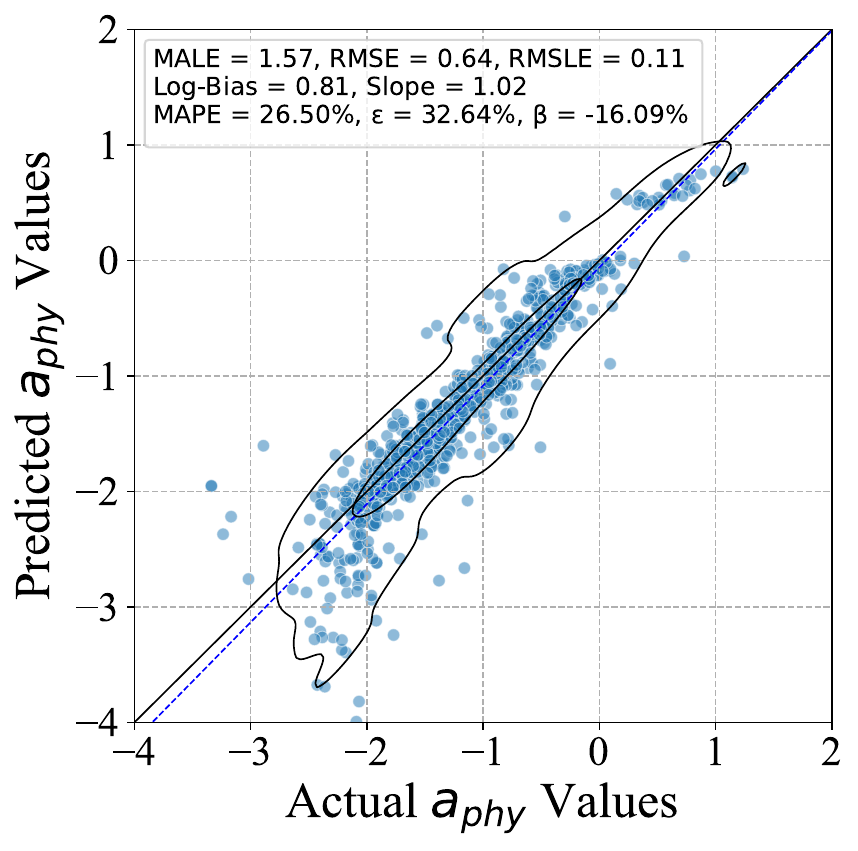}
		\label{Fig:EMIT_3_plots5}
	}	
	\subfigure[VAE on PACE 670nm]{
		\includegraphics[width=0.22\linewidth]{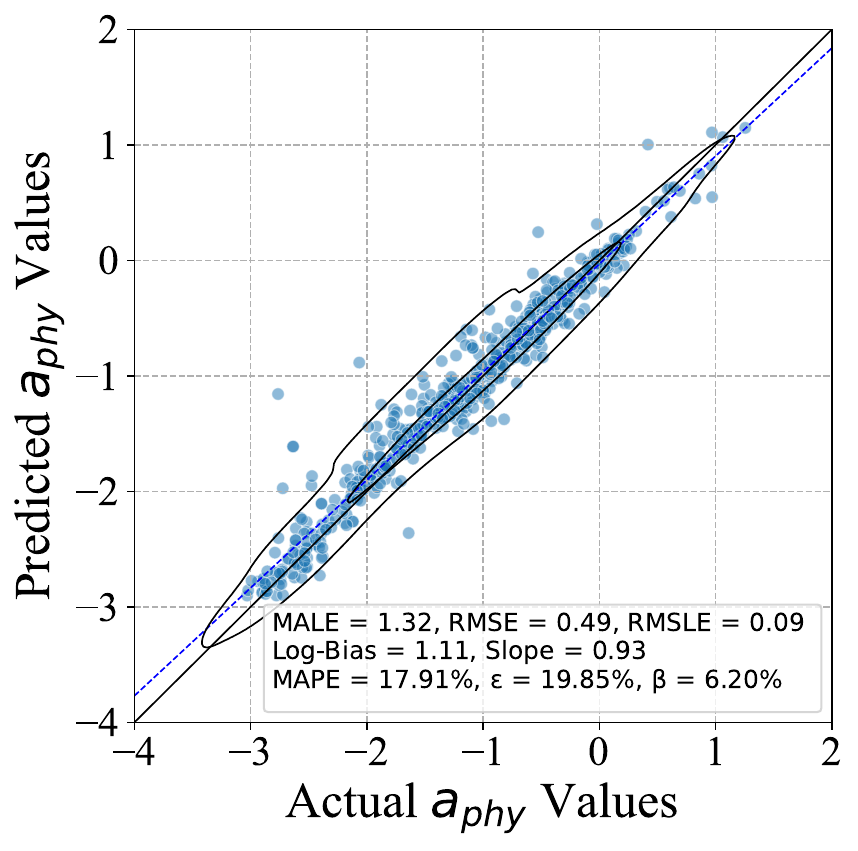}
		\label{Fig:PACE_3_plots3}
	}	
	\subfigure[MDN on PACE 670nm]{
		\includegraphics[width=0.22\linewidth]{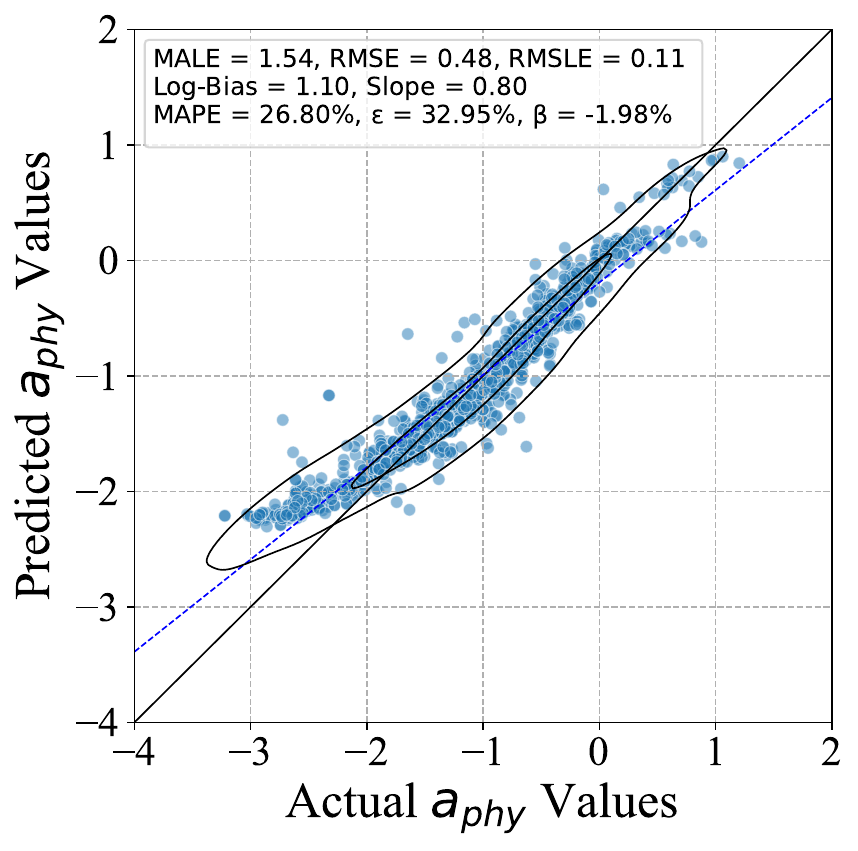}
		\label{Fig:PACE_3_plots6}
	}
 	\subfigure[VAE on EMIT 671nm]{
		\includegraphics[width=0.22\linewidth]{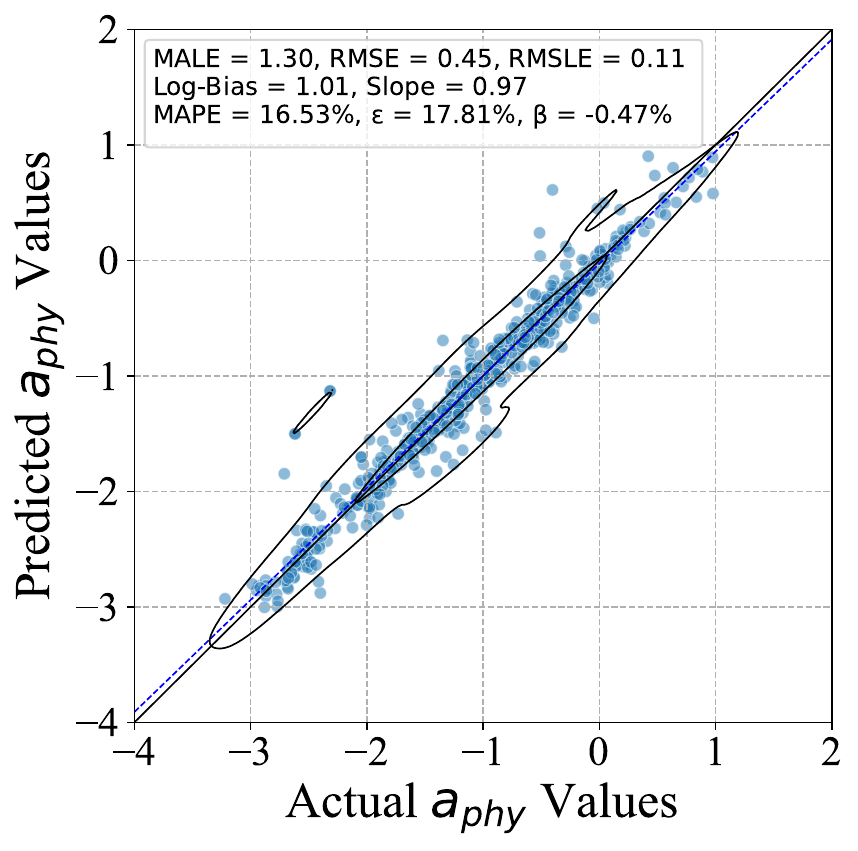}
		\label{Fig:EMIT_3_plots3}
	}	
	\subfigure[MDN on EMIT 671nm]{
		\includegraphics[width=0.22\linewidth]{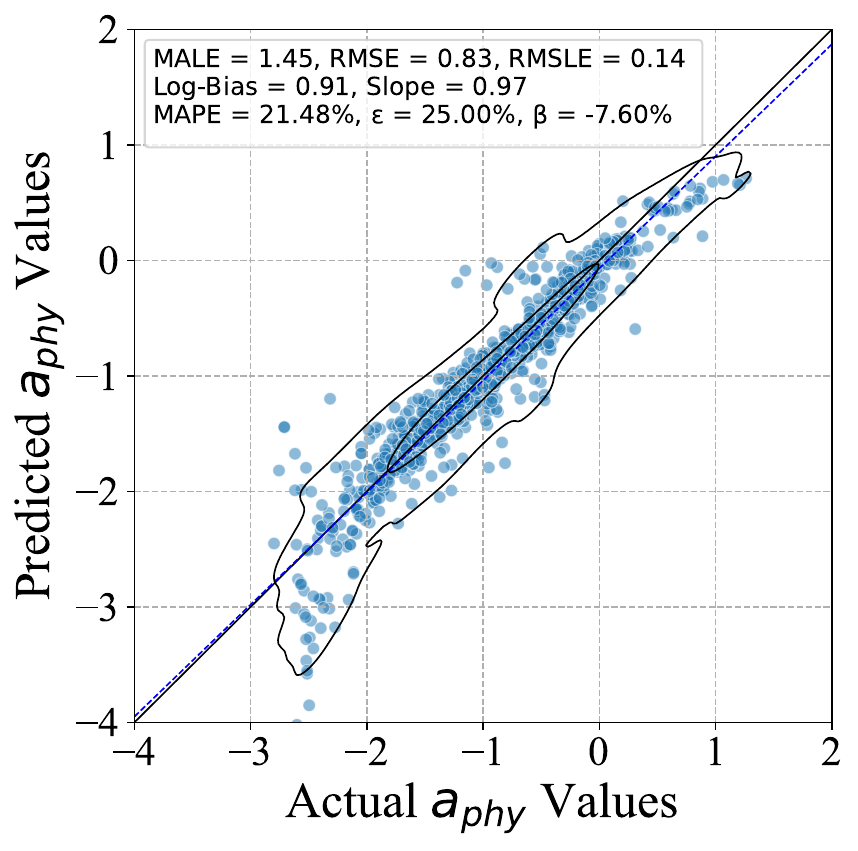}
		\label{Fig:EMIT_3_plots6}
	}
	\caption{Scatter plots and corresponding evaluation metrics for our VAE-$\mathit{a}_{ph}$ and MDN of $\mathit{a}_{ph}$ prediction tasks at three representative wavelengths for PACE and EMIT.}
	\label{fig:PACE_EMIT_plots}
\end{figure*}

\begin{figure*}[h]
	\centering
	\subfigure[Spectral distribution of the $R_{rs}$]{
		\includegraphics[width=0.4\linewidth]{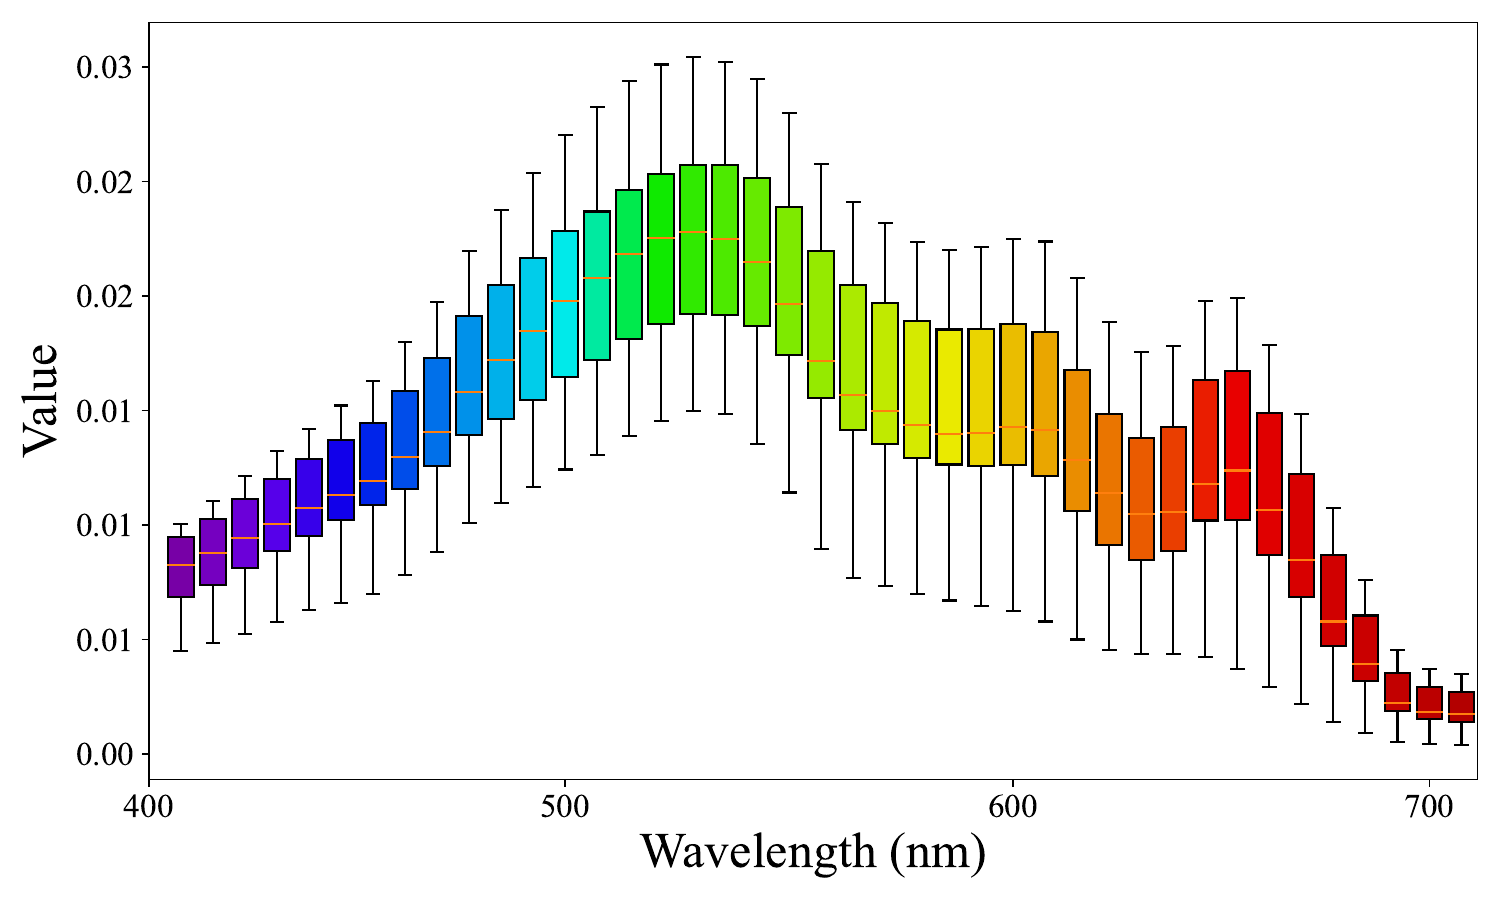}
		\label{Fig:EMIT_3_plots1}
	}	
	\subfigure[Spectral distribution of the $a_{phy}$]{
		\includegraphics[width=0.4\linewidth]{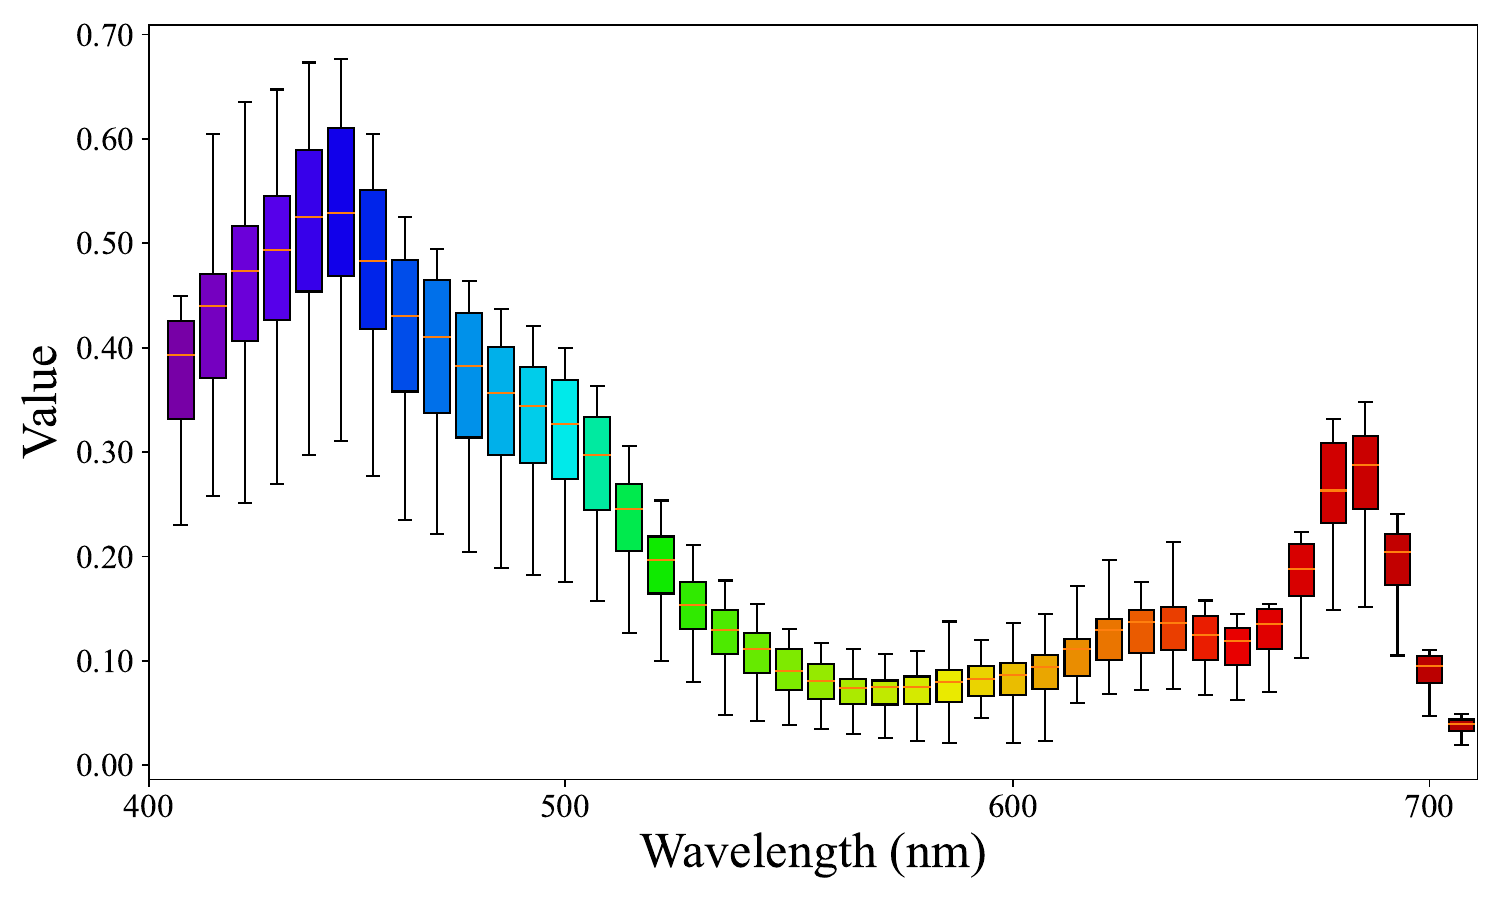}
		\label{Fig:EMIT_3_plots2}
	}
	\caption{Spectral distribution of the $R_{rs}$-$a_{phy}$ dataset, with bars denoting the minimum and maximum values for each EMIT band center.  }
	\label{fig:EMIT_3_plots}
\end{figure*}

\subsection{Results for Section 3.3}
\begin{figure*}[h]
	\centering
	\subfigure[VAE at Chla around 5.0 $\mu g\  L^{-1}$]{
		\includegraphics[width=0.3\linewidth]{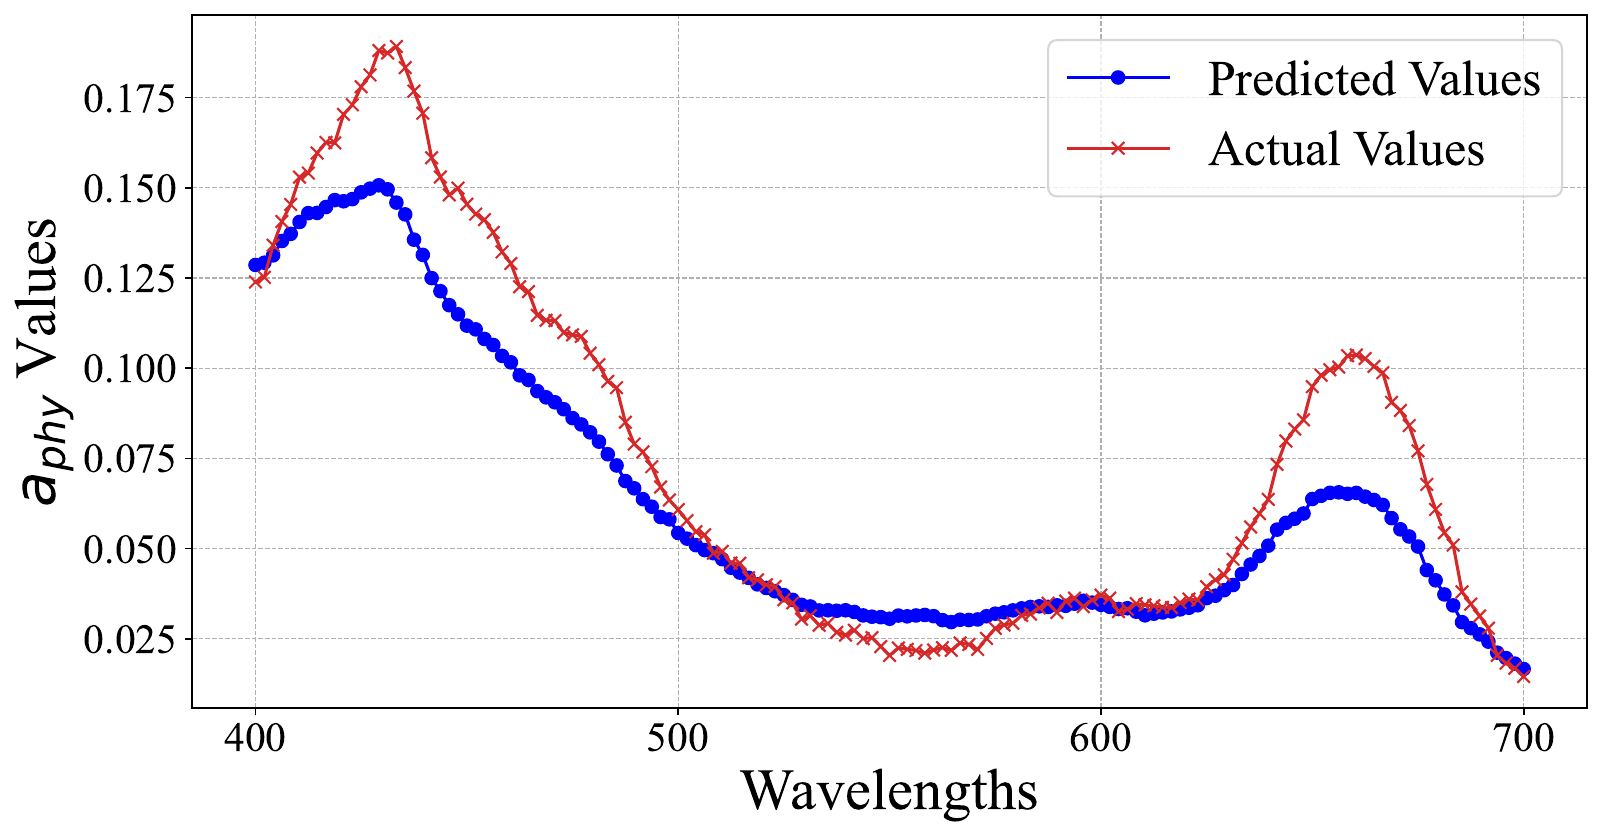}
		\label{Fig:EMIT_3_plots1}
	}	
	\subfigure[VAE at Chla around 30.0 $\mu g\  L^{-1}$]{
		\includegraphics[width=0.3\linewidth]{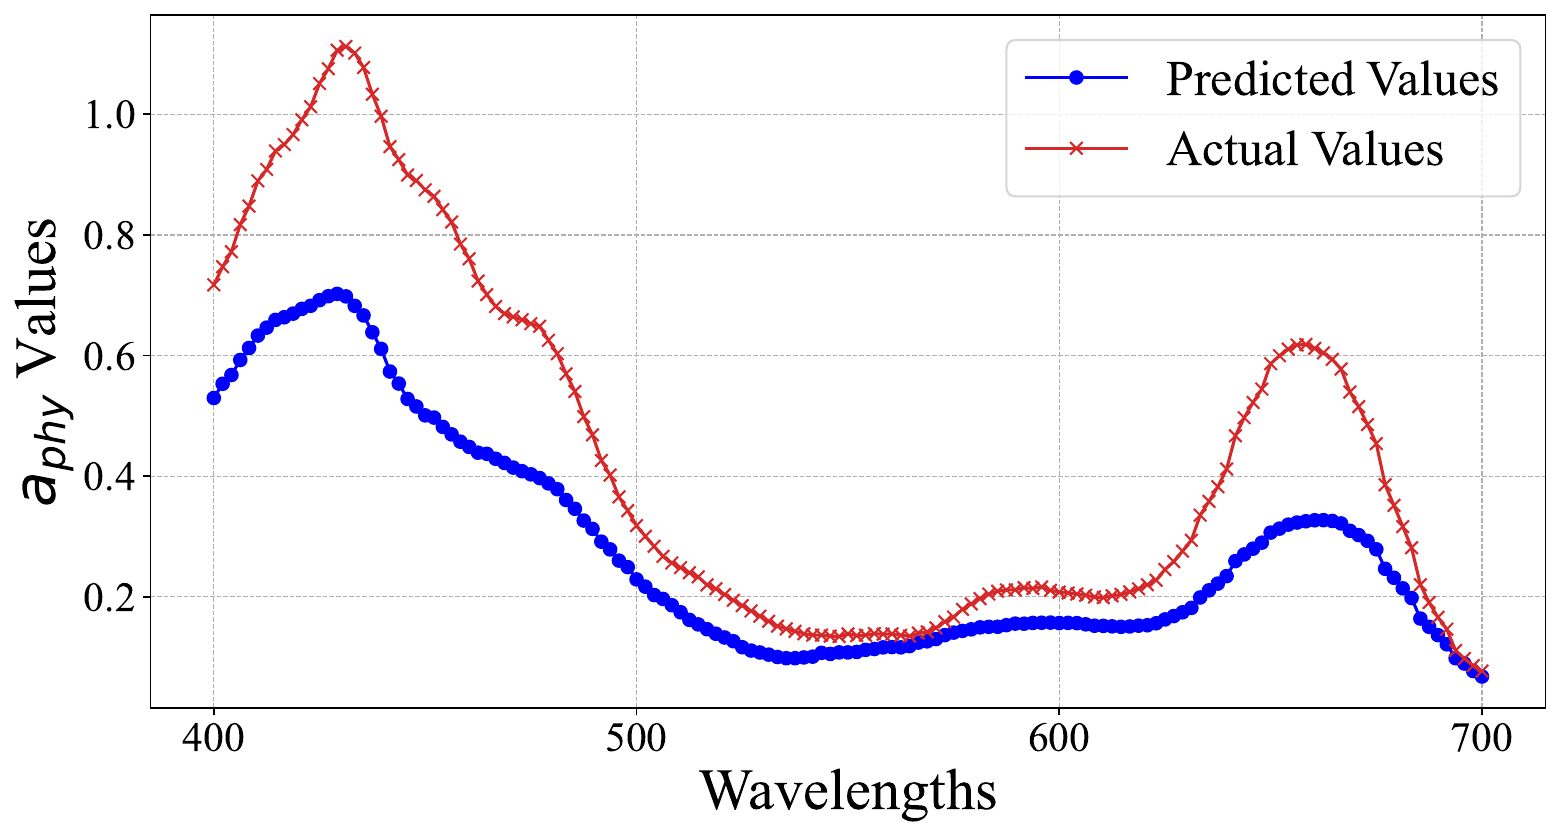}
		\label{Fig:EMIT_3_plots2}
	}
	\subfigure[VAE at Chla around 50.0 $\mu g\  L^{-1}$]{
		\includegraphics[width=0.3\linewidth]{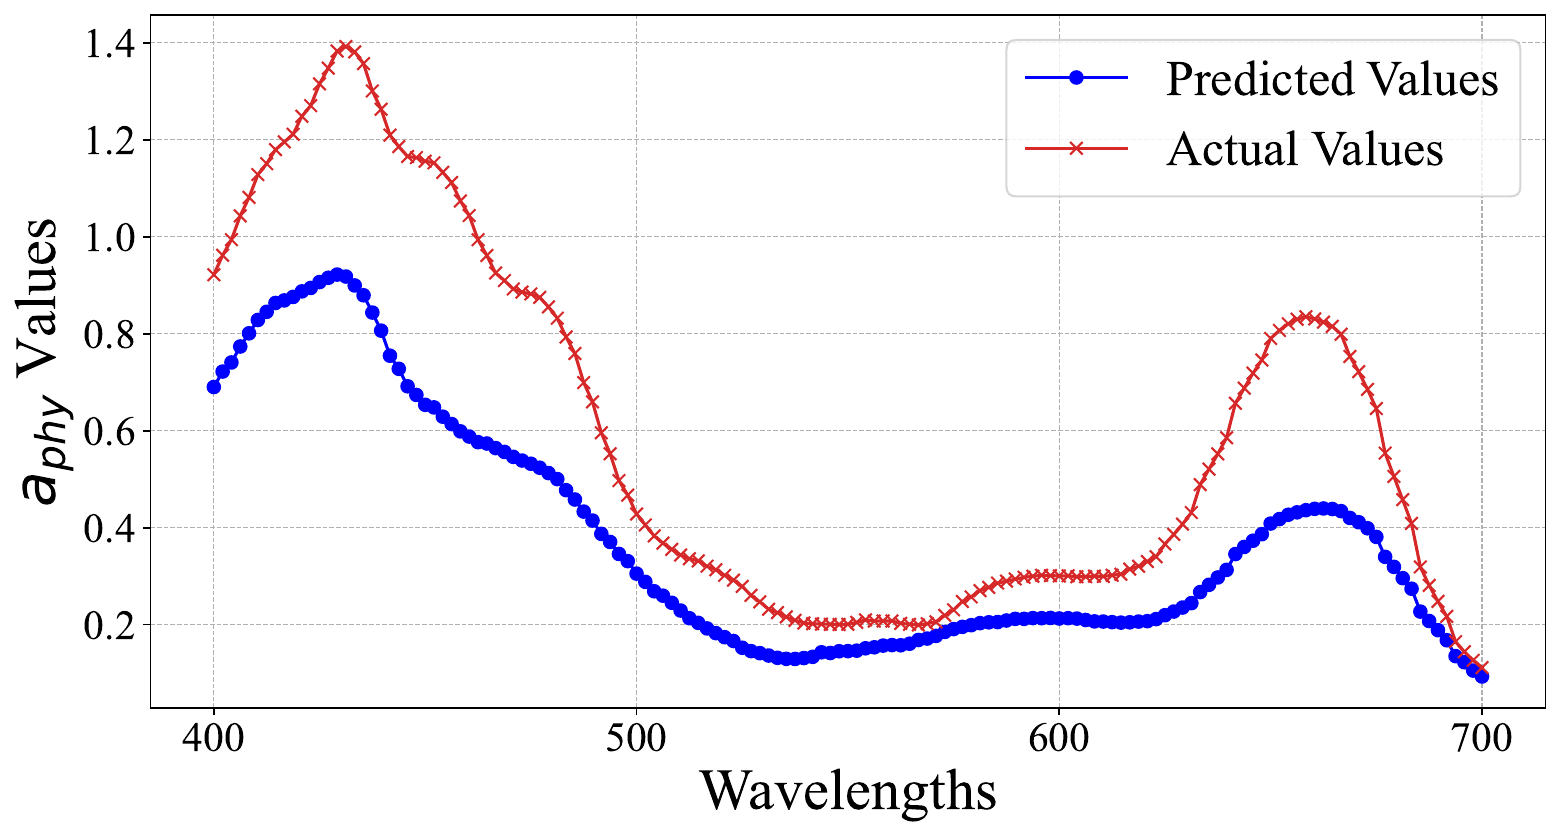}
		\label{Fig:EMIT_3_plots3}
	}	
	\subfigure[MDN at Chla around 5.0 $\mu g\  L^{-1}$]{
		\includegraphics[width=0.3\linewidth]{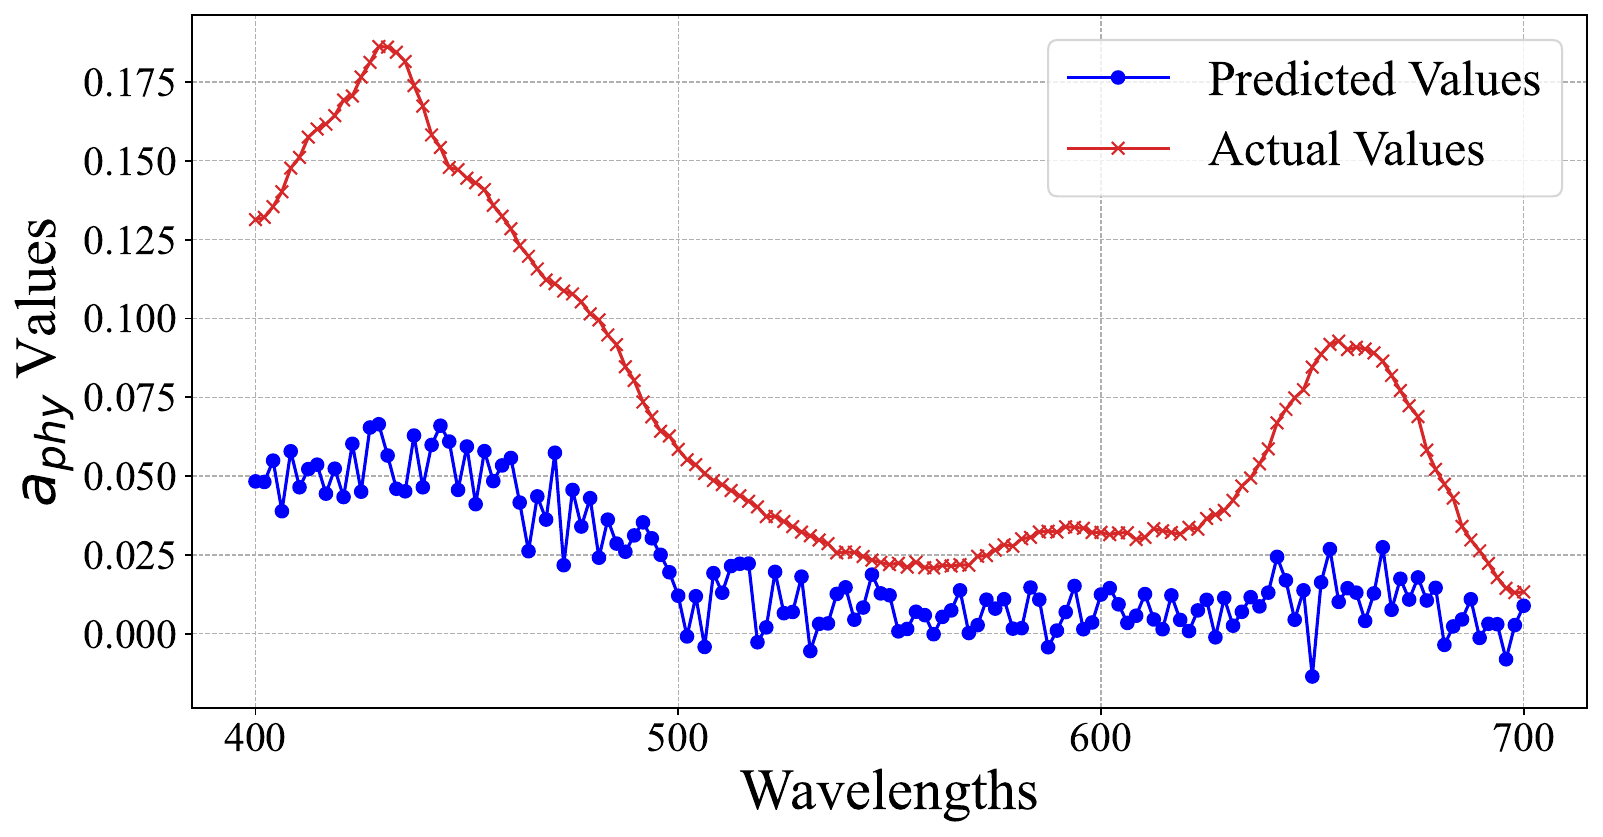}
		\label{Fig:EMIT_3_plots4}
	}
	\subfigure[MDN at Chla around 30.0 $\mu g\  L^{-1}$]{
		\includegraphics[width=0.3\linewidth]{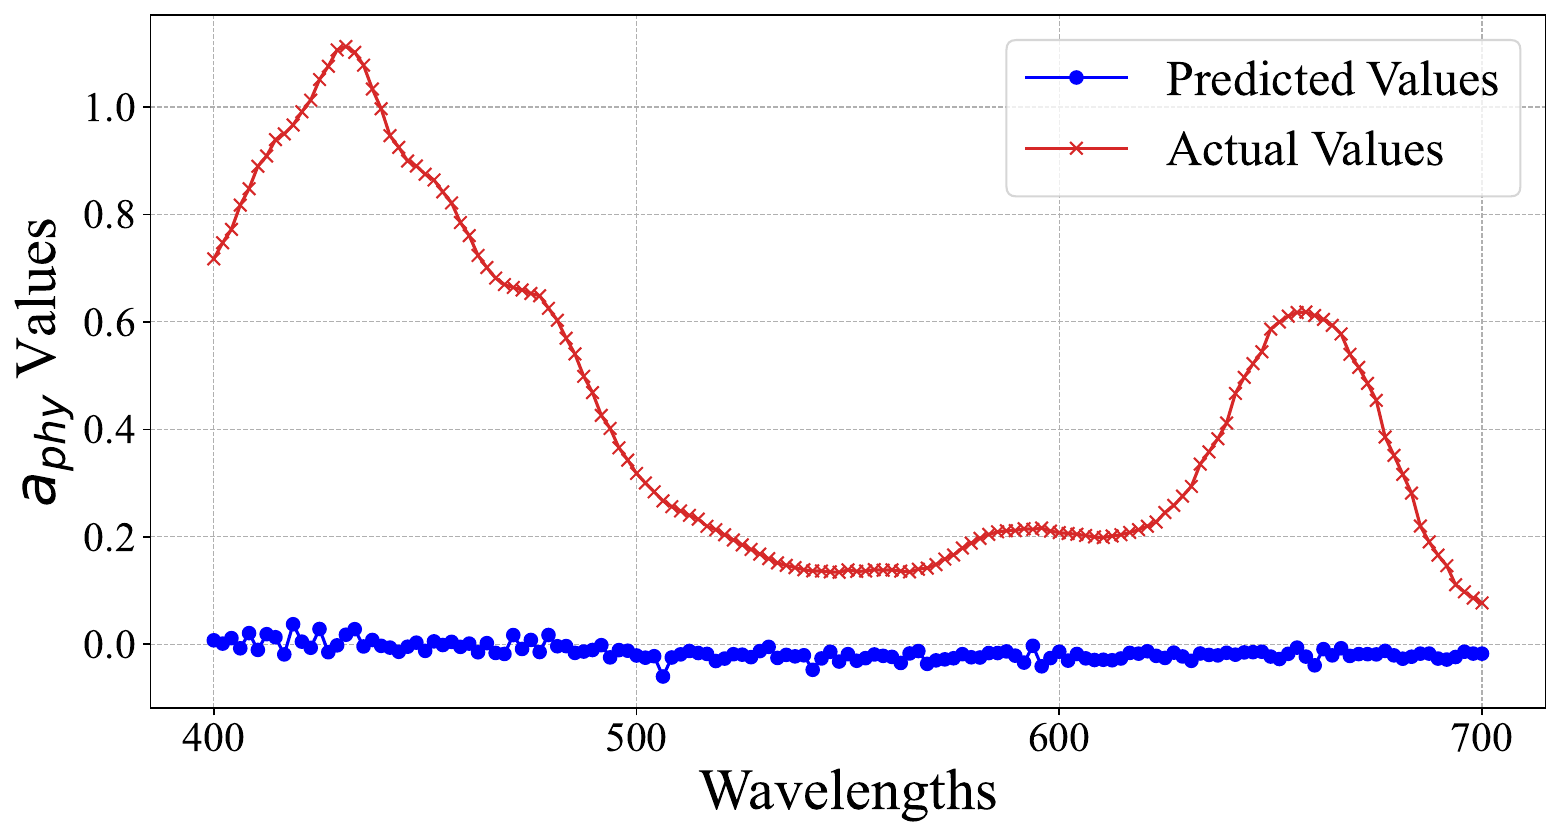}
		\label{Fig:EMIT_3_plots5}
	}	
	\subfigure[MDN at Chla around 50.0 $\mu g\  L^{-1}$]{
		\includegraphics[width=0.3\linewidth]{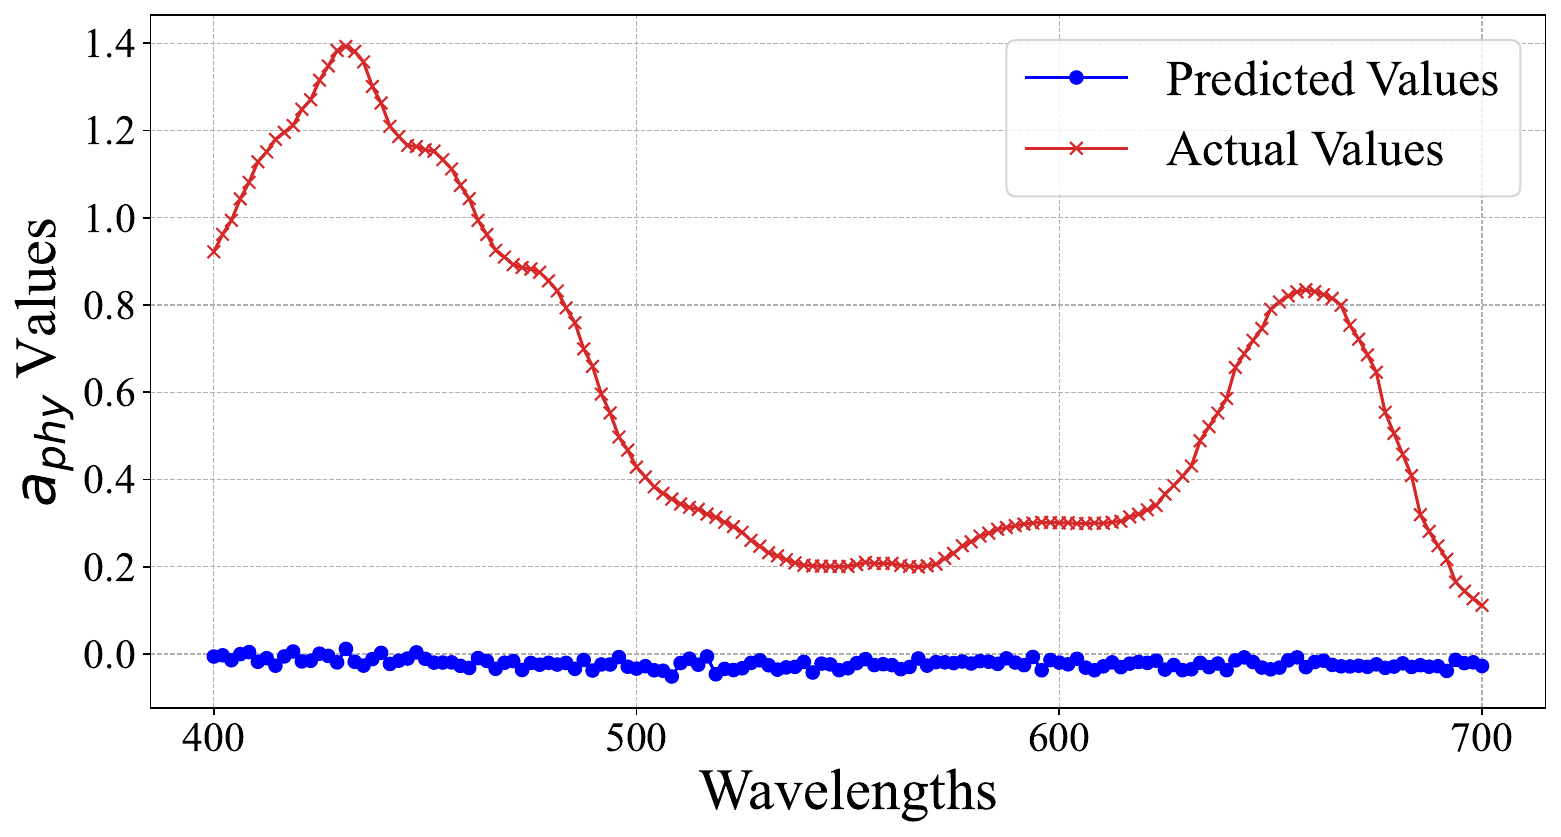}
		\label{Fig:EMIT_3_plots6}
	}
	\caption{The actual and predicted $a_{phy}$  spectra across the 400nm-700nm wavelengths at PACE waveband under different Chla levels}
	\label{fig:EMIT_3_plots}
\end{figure*}

\begin{figure*}[h]
	\centering
	\subfigure[VAE at Chla around 5.0 $\mu g\  L^{-1}$]{
		\includegraphics[width=0.3\linewidth]{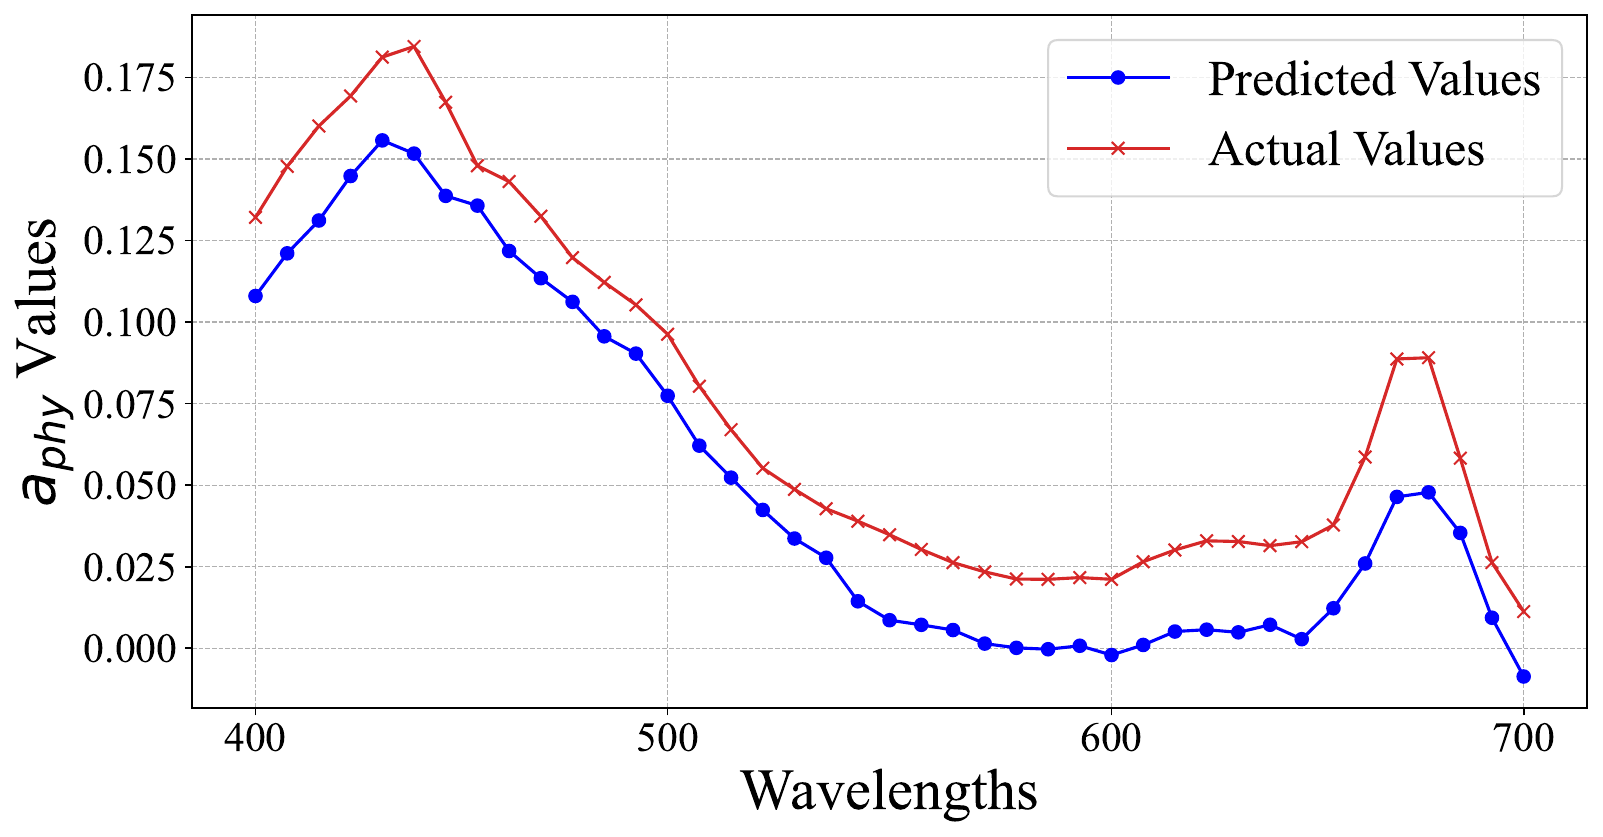}
		\label{Fig:EMIT_3_plots1}
	}	
	\subfigure[VAE at Chla around 30.0 $\mu g\  L^{-1}$]{
		\includegraphics[width=0.3\linewidth]{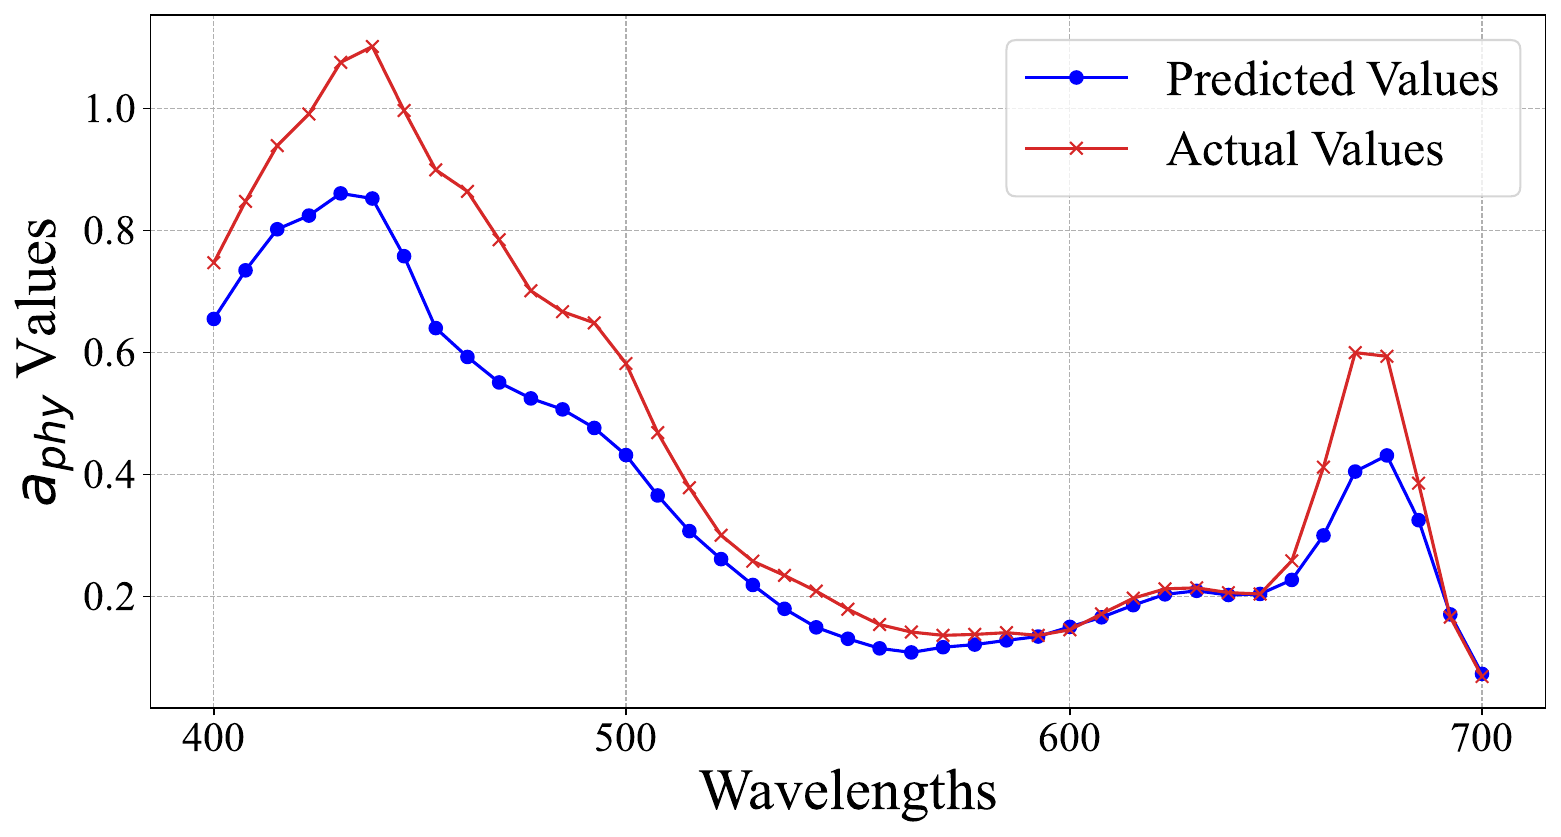}
		\label{Fig:EMIT_3_plots2}
	}
	\subfigure[VAE at Chla around 50.0 $\mu g\  L^{-1}$]{
		\includegraphics[width=0.3\linewidth]{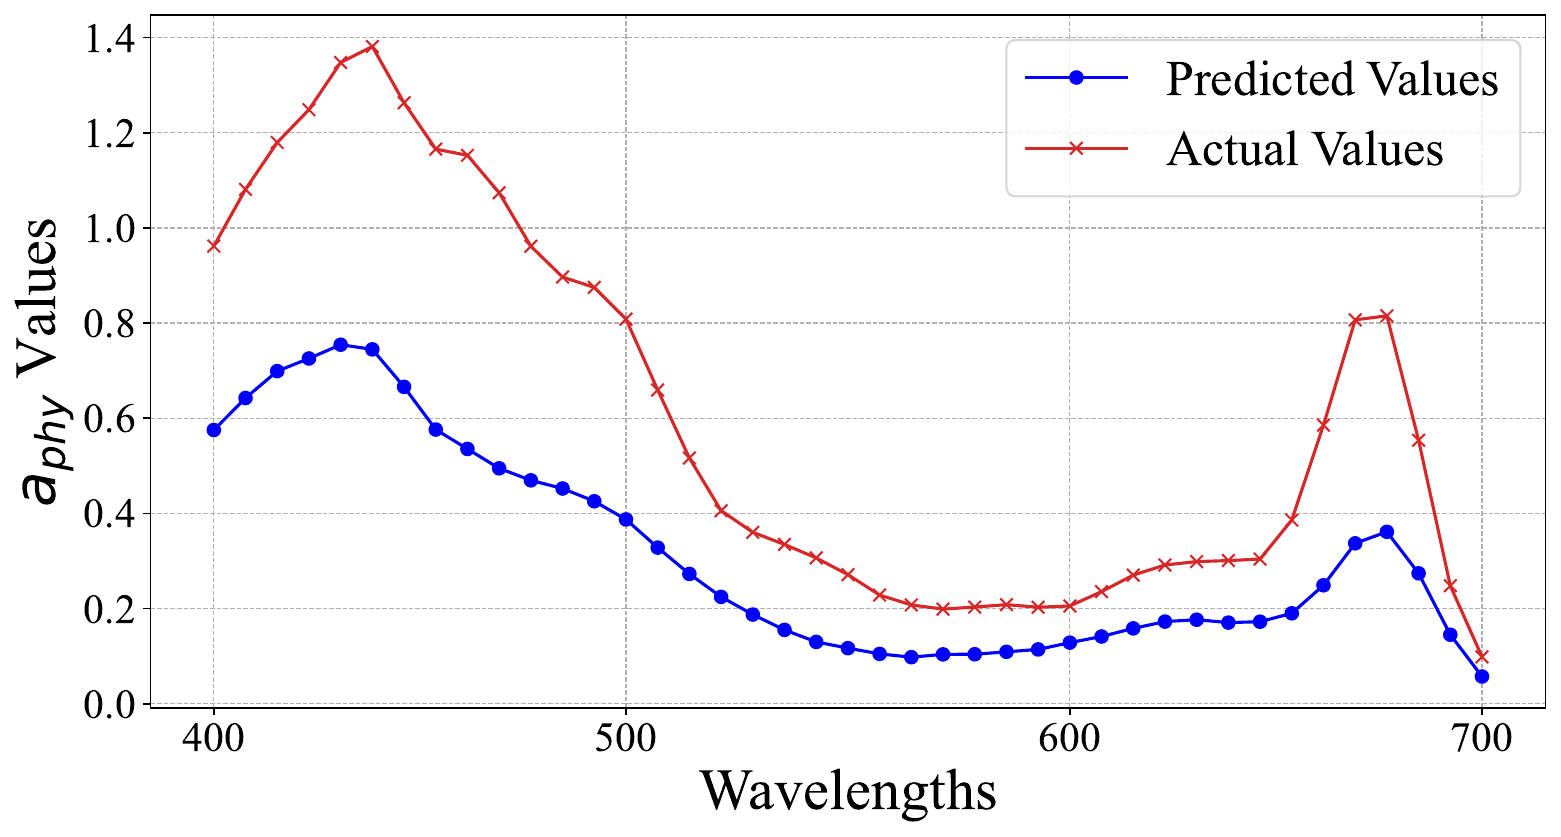}
		\label{Fig:EMIT_3_plots3}
	}	
	\subfigure[MDN at Chla around 5.0 $\mu g\  L^{-1}$]{
		\includegraphics[width=0.3\linewidth]{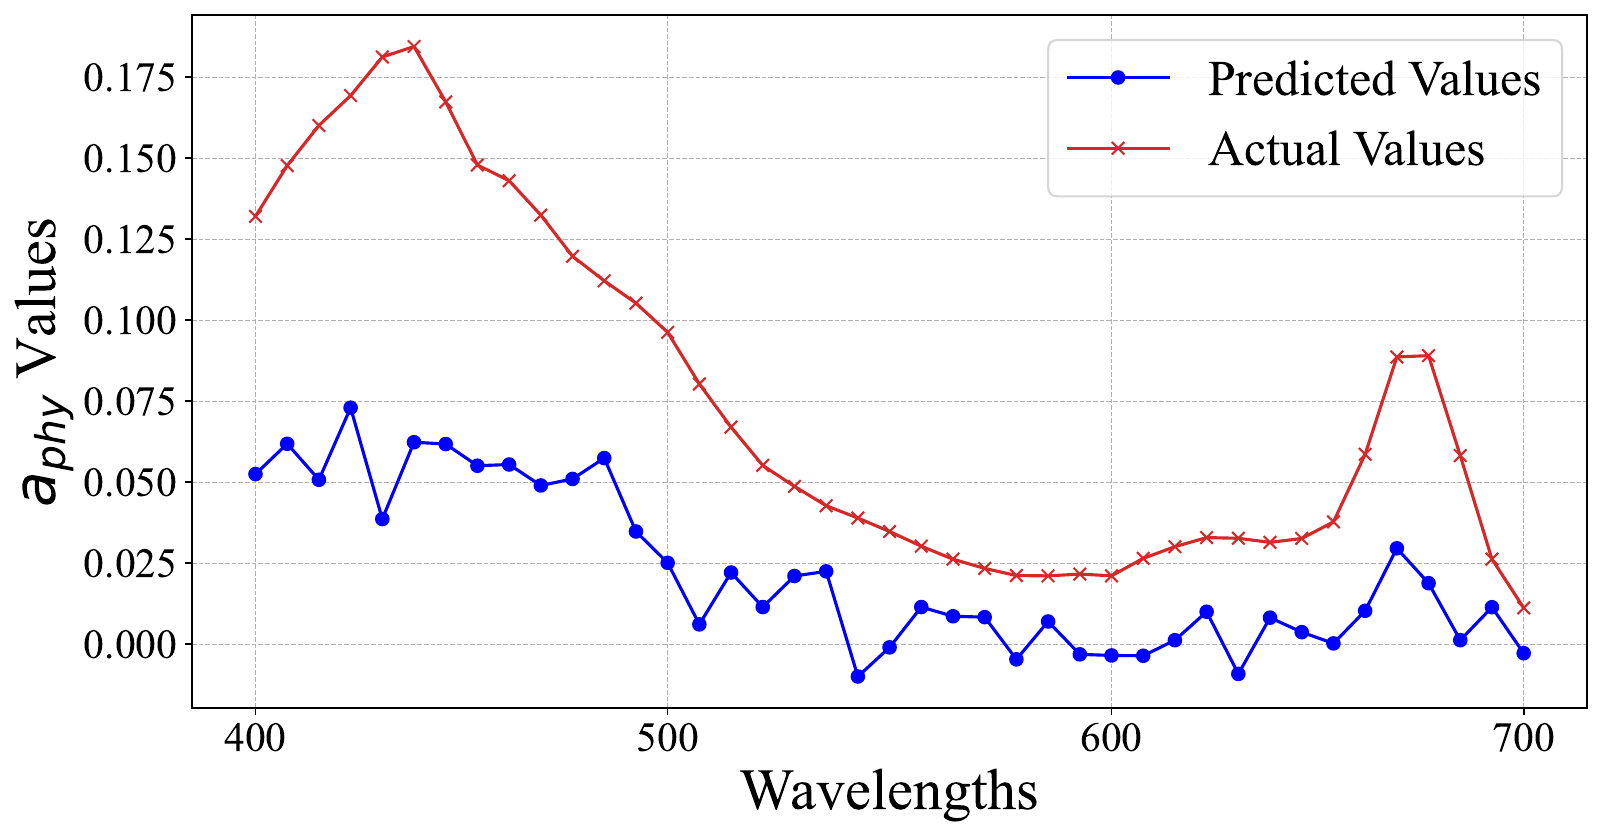}
		\label{Fig:EMIT_3_plots4}
	}
	\subfigure[MDN at Chla around 30.0 $\mu g\  L^{-1}$]{
		\includegraphics[width=0.3\linewidth]{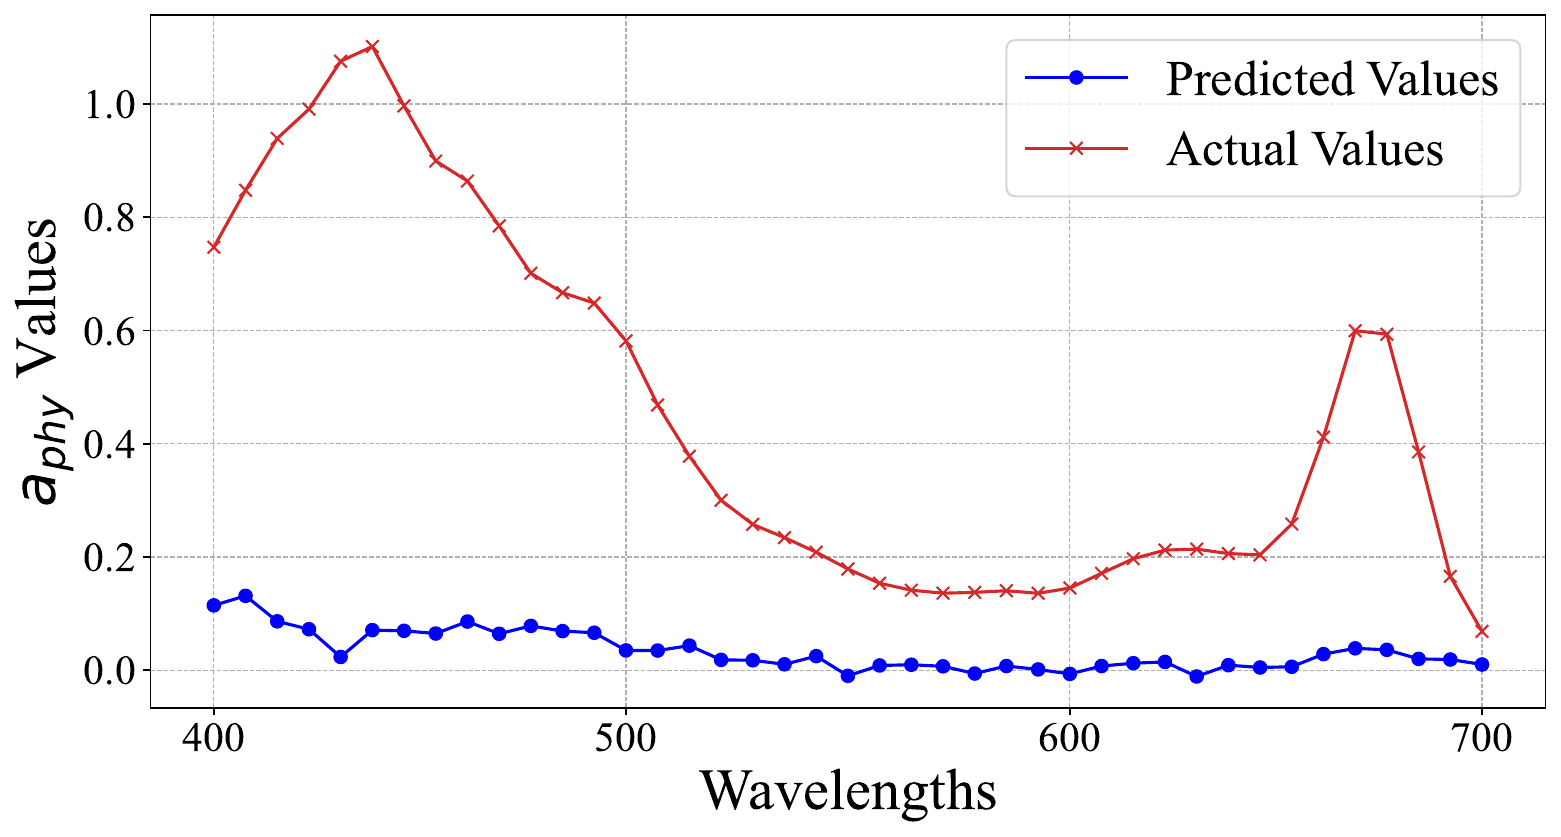}
		\label{Fig:EMIT_3_plots5}
	}	
	\subfigure[MDN at Chla around 50.0 $\mu g\  L^{-1}$]{
		\includegraphics[width=0.3\linewidth]{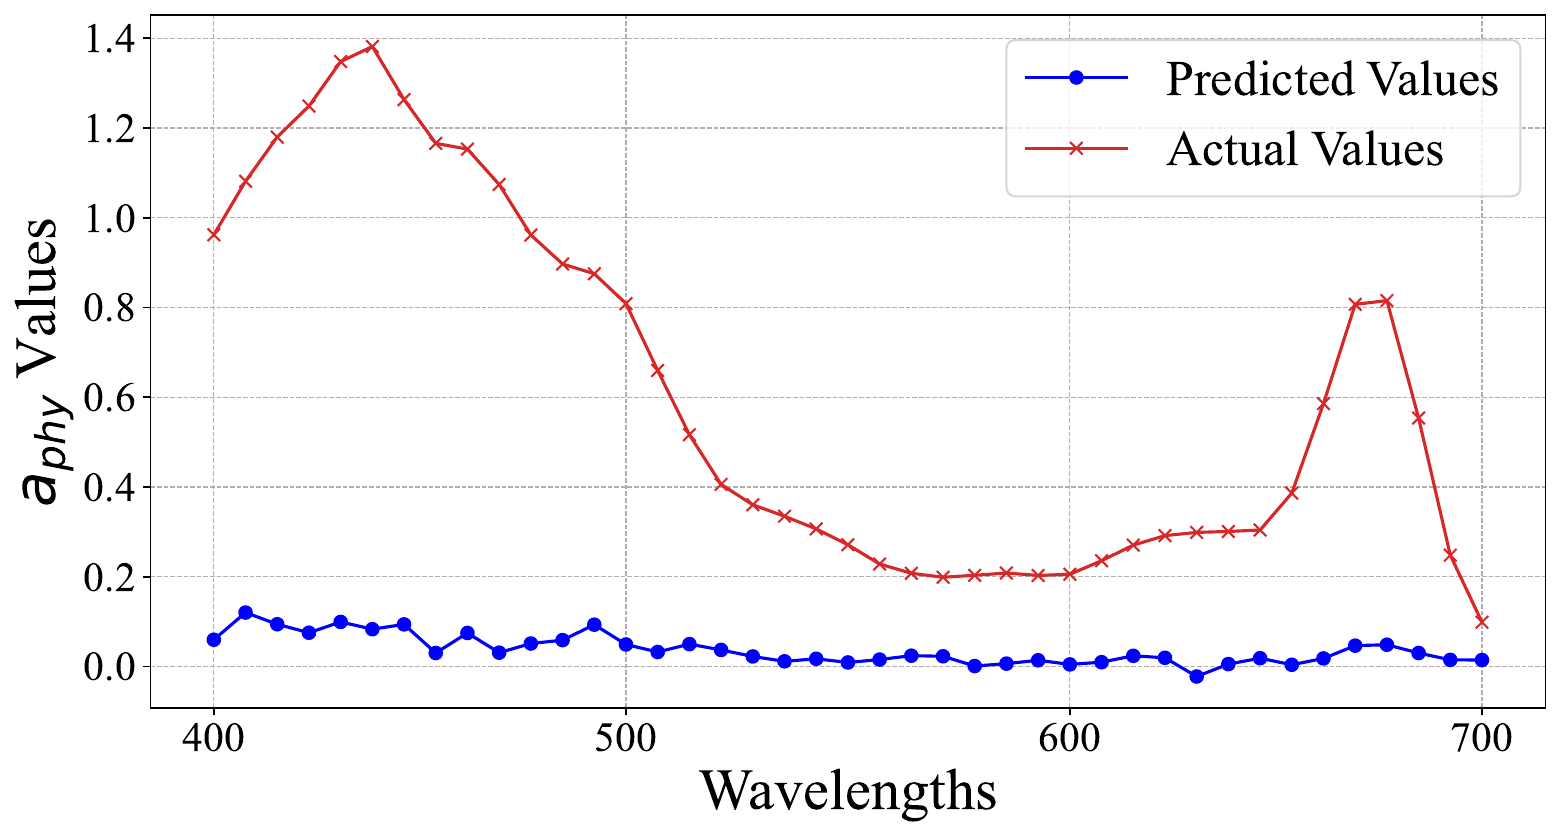}
		\label{Fig:EMIT_3_plots6}
	}
	\caption{The actual and predicted $a_{phy}$  spectra across the 400nm-700nm wavelengths at EMIT waveband under different Chla levels}
	\label{fig:EMIT_3_plots}
\end{figure*}

\begin{figure*}
	\centering
	\subfigure[444nm wavelength under 40 bins.]{
		\includegraphics[width=0.30\linewidth]{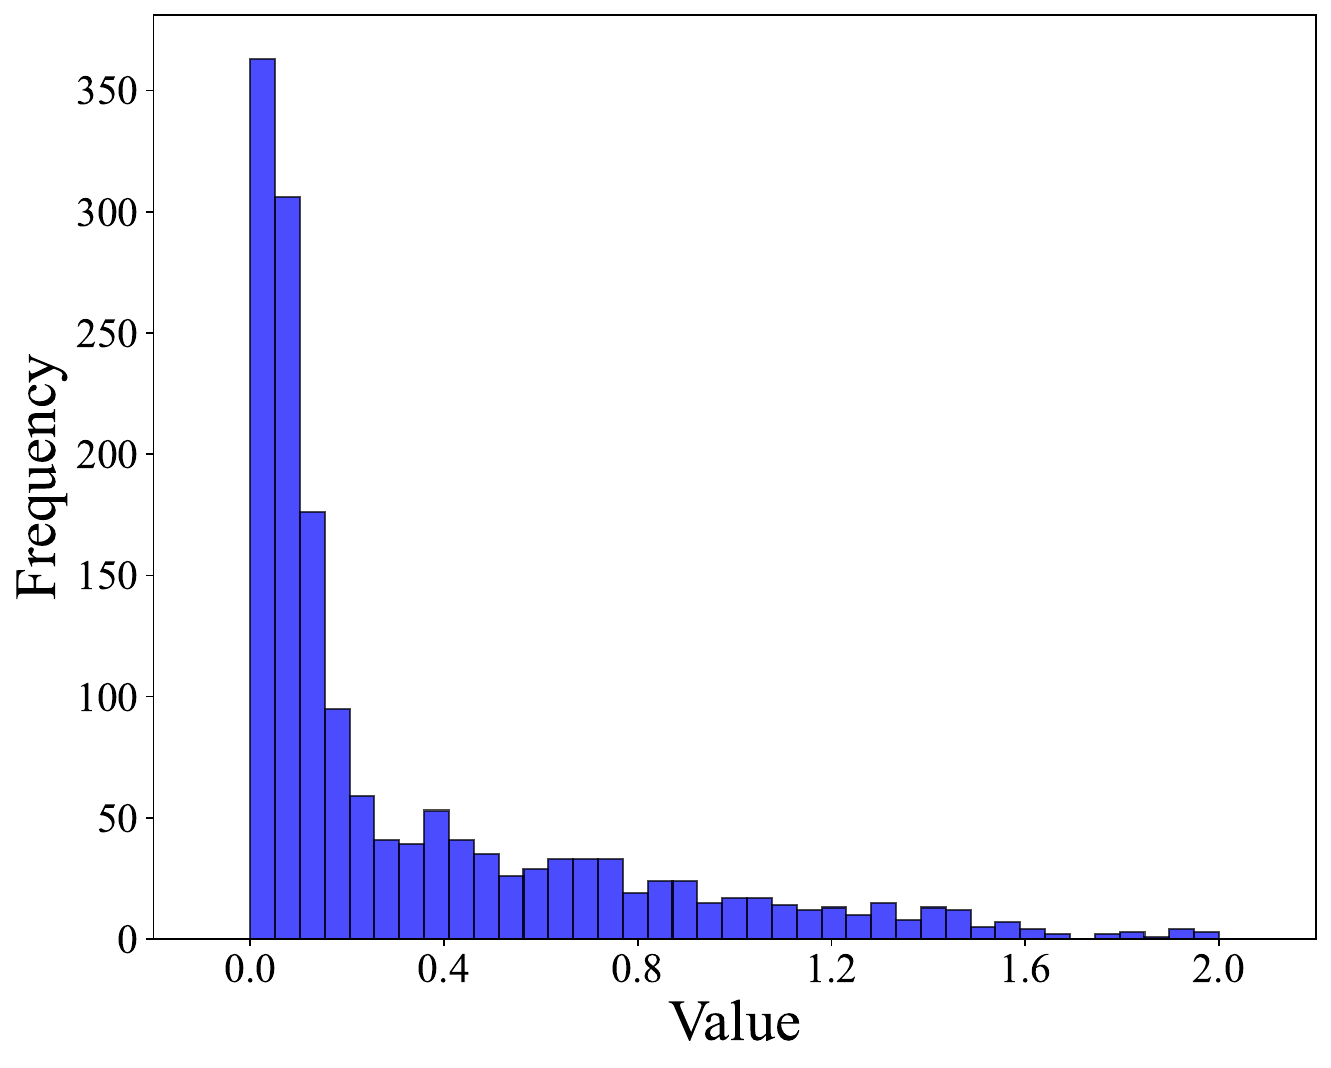}
		\label{Fig:dis:444:40}
	}	
	\subfigure[444nm wavelength under 100 bins.]{
		\includegraphics[width=0.30\linewidth]{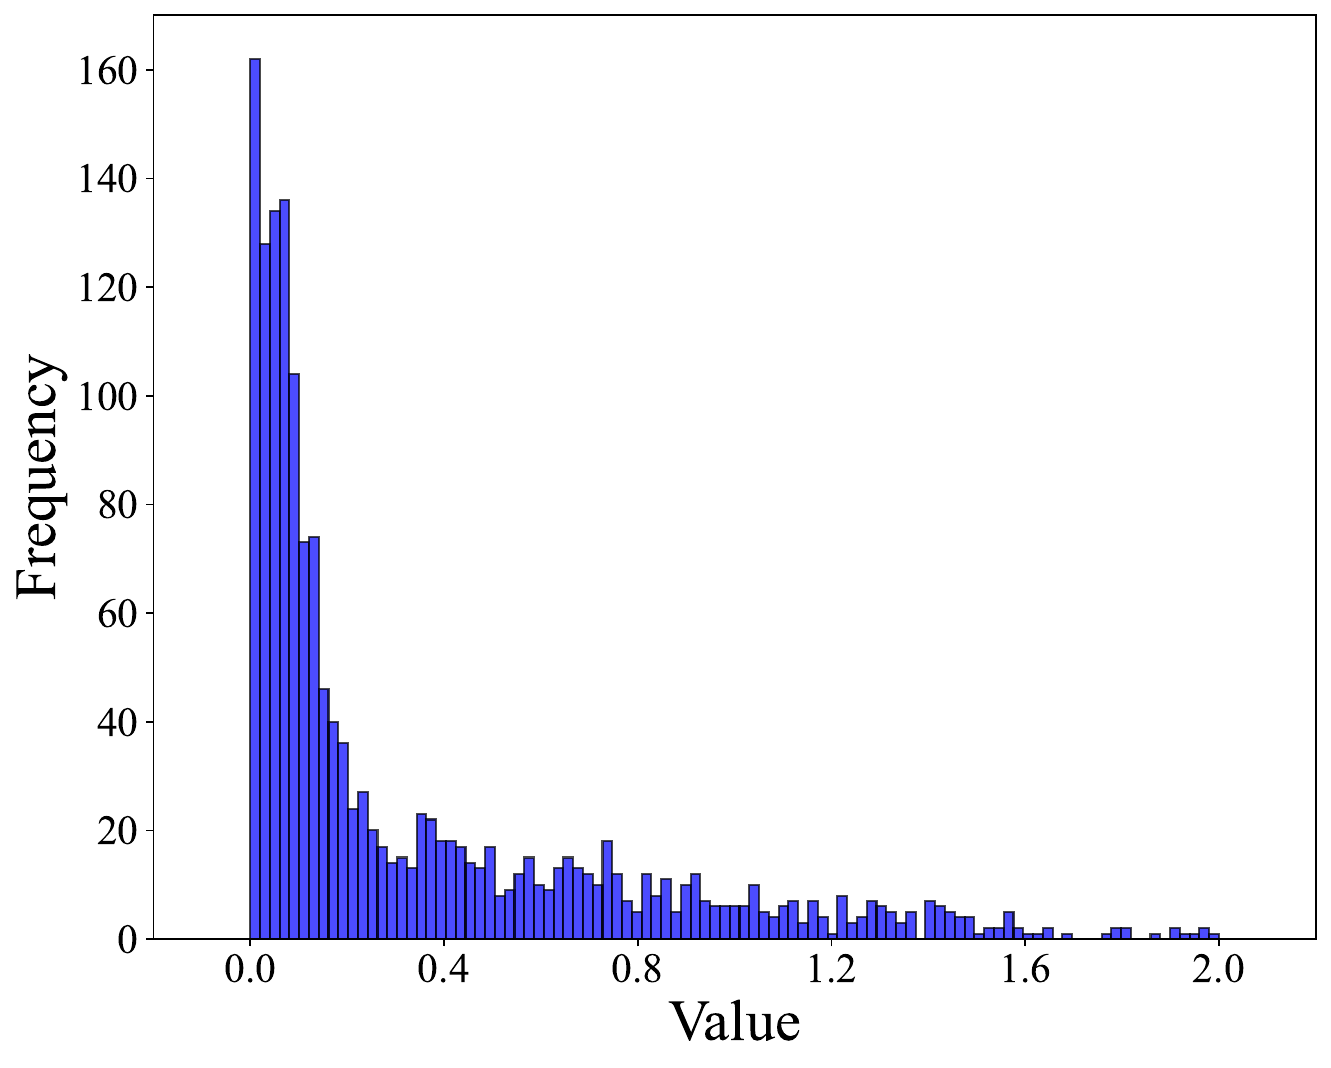} 
            \label{{Fig:dis:444:100}}
            }
        \subfigure[621nm wavelength under 40 bins.]{
		\includegraphics[width=0.30\linewidth]{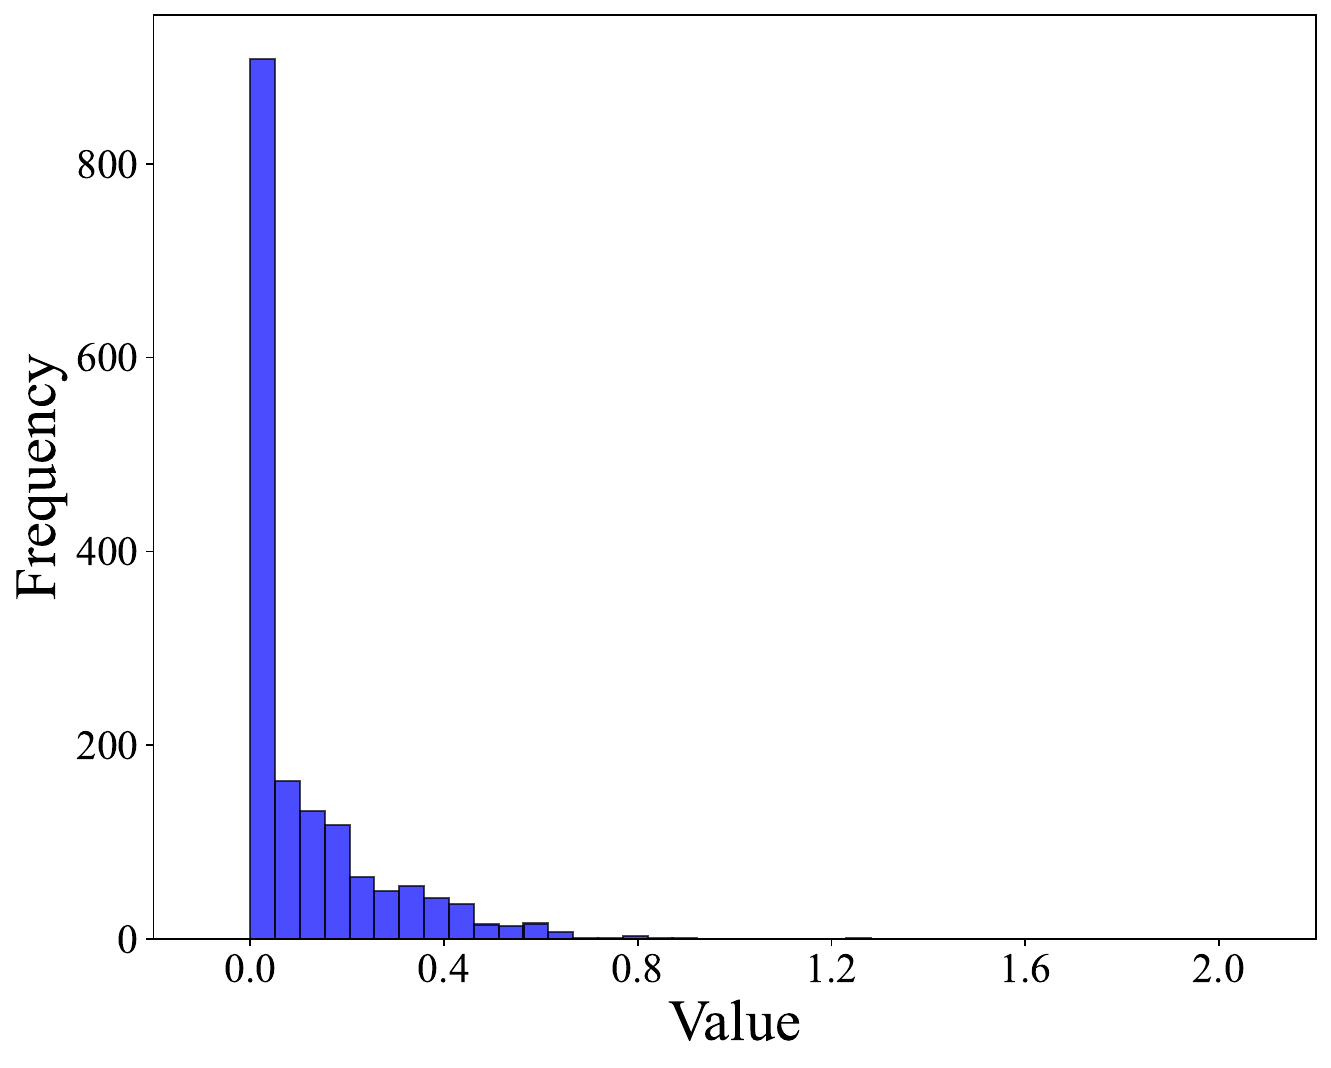}
		\label{Fig:dis:621:40}
	}	
	\caption{The $\mathit{a}_{phy}$ distribution under different wavelength.}
	\label{Fig:dis}
\end{figure*}

\begin{figure*}
	\centering
	\subfigure[444nm wavelength under 100 bins.]{
		\includegraphics[width=0.30\linewidth]{figs/Rrs_444.pdf}
		\label{Fig:dis:444:100}
	}	
	\subfigure[673nm wavelength under 100 bins.]{
		\includegraphics[width=0.30\linewidth]{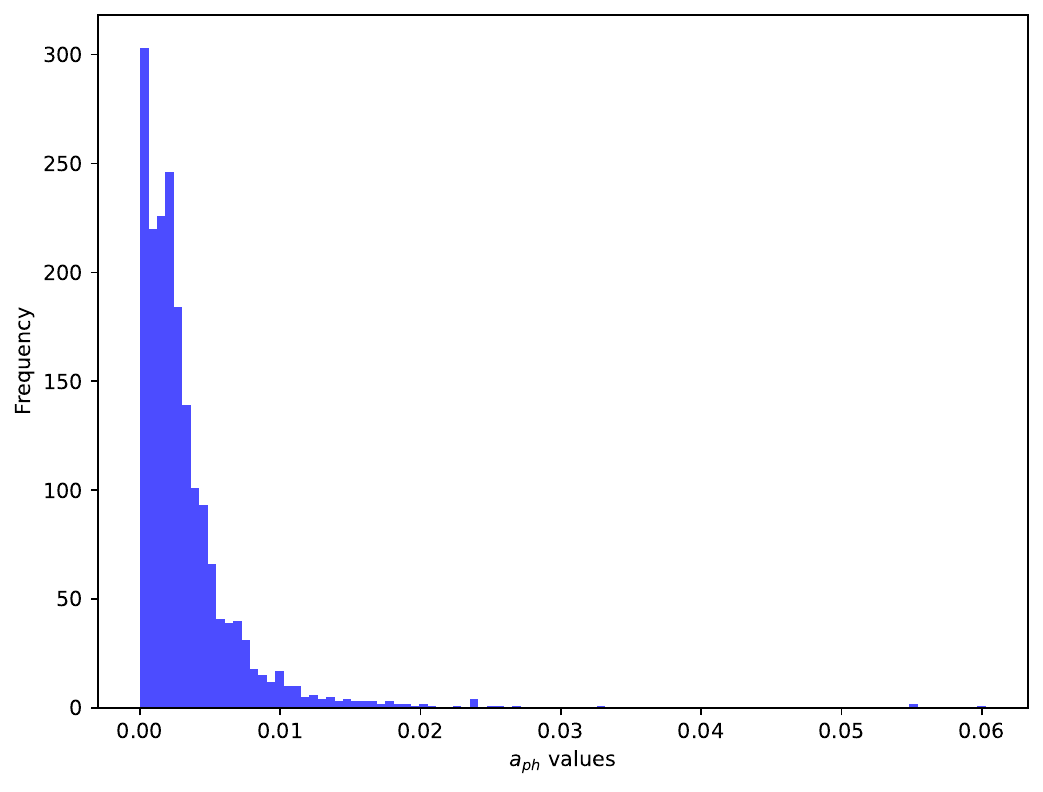} 
            \label{{Fig:dis:673:100}}
            }
        \subfigure[444nm wavelength under 300 bins.]{
		\includegraphics[width=0.30\linewidth]{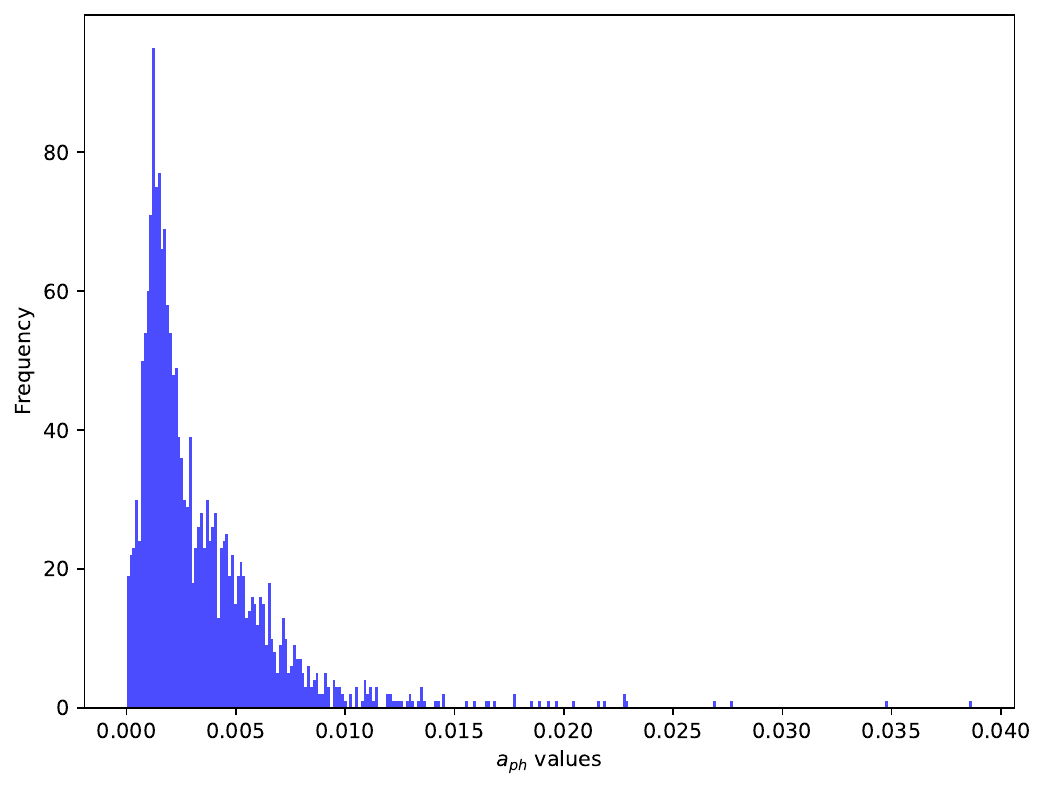}
		\label{Fig:dis:444:300}
	}	
	\caption{The $\mathit{a}_{phy}$ distribution under different wavelength.}
	\label{Fig:dis}
\end{figure*}

\subsection{Comparisons of Generality for $\aphy$ Predictions between VAE and MDN}
We further assess robustness and generality of the trained VAE-$\aphy$ and MDN models by testing them on a separate in-situ dataset from Galveston Bay, TX, USA, that the models have not encountered during training to verify the models’ ability to generalize $\aphy$ estimation. 
The TX in-situ dataset features $\Rrs$- $\aphy$  samples with high Chl a concentrations, collected from algal bloom waters dominated by cryptophyte~\cite{liu2019floodwater}. 
This condition was underrepresented in the training data. Figs. 10 and 11 present the actual and predicted $\aphy$ spectra across the 400-700 nm at PACE and EMIT wavebands, corresponding to low (5.0 $\mu$ g $L^{-1}$), medium (30.0 $\mu$g $L^{-1}$), and high (50.0 $\mu$g $L^{-1}$) Chl a concentrations, evaluating how well the VAE and MDN models generalize across different geographic locations and varying Chl a levels. We continue to observe robust estimations from VAE-$\aphy$model, which outperforms MDN in predicting $\aphy$ spectra (Figs. 10 and 11) at three Chl a levels. 
The $\aphy$ predictions from the VAE-$\aphy$ model align well with the actual values across all wavelengths, while MDN predictions exhibit zigzag lines, indicating instability (Figs. 10 and 11). 
This difference in performance is due to the VAE’s advanced learning structure, which does not directly fit the $\aphy$ distribution from the training data, but instead learns a Gaussian distribution to capture the high-level patterns in the $\Rrs$-$\aphy$ relationship for predictions. 
It is observed that VAE-$\aphy$ performs well in predicting $\aphy$ at the higher Chl a concentrations, such as, 30 and 50 $\mu$g $L^{-1}$, compared to lower Chl a levels (e.g., 5.0 $\mu$g $L^{-1}$; Figs. 10 and 11), which could be attributed to underrepresentation of this water type included in the training datasets. 
This lower Chl a site was located at the entrance of Galveston Bay where it connects to the relatively clear seawaters of the northern Gulf of Mexico, is expected to exhibit different optical properties from those of the training dataset in [6] and other sites in the TX dataset~\cite{liu2019floodwater}. 
This difference might constrain the models' ability to learn these relevant patterns, resulting in reduced estimation accuracy for both MDN and VAE-$\aphy$ models (e.g., Figs. 10a and 10d). 
While VAE-$\aphy$ predictions accurately capture the magnitude of $\aphy$ spectra at where Chl a reach 30 and 50 $\mu$g $L^{-1}$, it is worth noting that a few minor absorption peaks associated with other pigments, such as Chl b, Chl c, and carotenoids in the 450-500 nm range (Figs. 10c and 11c) are missing from the predictions~\cite{bricaud2004natural}. 
This suggests that while VAE-$\aphy$ performs well overall, the training dataset may not be comprehensive enough to fully capture the diversity of water types, such as algal blooms. These experimental results are critical and underscore the practical advantages of using VAE over MDN, such as improved generality on unseen geolocation data and greater stability across wavelengths. At the same time, they highlight areas for improvement to enhance its applications in hyperspectral ocean color remote sensing.
